# Supplementary material for: The enriched $q$-monomial basis of the quasisymmetric functions
Source: arXiv:2309.01118 ancillary file (2026-06-05)
Supplement: Supplementary file 1 [file comps-compiled.pdf]

# Some basic properties of compositions

Darij Grinberg and Ekaterina A. Vassilieva

June 14, 2024

## Contents

|                                                |    |
|------------------------------------------------|----|
| 1. Notations                                   | 1  |
| 2. The maps $D$ and $\text{comp}$              | 2  |
| 3. Reversals                                   | 6  |
| 4. The omega operation                         | 15 |
| 5. Concatenation                               | 20 |
| 5.1. Definition and basic properties . . . . . | 20 |
| 5.2. Concatenation and reversal . . . . .      | 21 |
| 5.3. Concatenation and partial sums . . . . .  | 21 |
| 5.4. Further lemmas . . . . .                  | 29 |
| 5.5. Concatenation and coarsenings . . . . .   | 34 |

\*\*\*

This is a companion note to [GriVas22]. The purpose of this note is to prove some elementary properties of integer compositions that are used in [GriVas22]. All of these proofs are elementary and generally quite easy, but they are hard to find written down and often left to the reader to prove.

## 1. Notations

We let  $\mathbb{N} = \{0, 1, 2, \dots\}$ .

A *composition* means a finite list  $(\alpha_1, \alpha_2, \dots, \alpha_k)$  of positive integers. The set of all compositions will be denoted by  $\text{Comp}$ .

The *empty composition* is defined to be the composition  $()$ , which is a 0-tuple. It is denoted by  $\emptyset$ .

The *length*  $\ell(\alpha)$  of a composition  $\alpha = (\alpha_1, \alpha_2, \dots, \alpha_k)$  is defined to be the number  $k$ .

If  $\alpha = (\alpha_1, \alpha_2, \dots, \alpha_k)$  is a composition, then the nonnegative integer  $\alpha_1 + \alpha_2 + \dots + \alpha_k$  is called the *size* of  $\alpha$  and is denoted by  $|\alpha|$ . For any  $n \in \mathbb{N}$ , we define a *composition of  $n$*  to be a composition that has size  $n$ . We let  $\text{Comp}_n$  be the set of all compositions of  $n$  (for given  $n \in \mathbb{N}$ ). The notation " $\alpha \models n$ " is short for " $\alpha \in \text{Comp}_n$ ". For example,  $(1, 5, 2, 1)$  is a composition with size 9 (since  $|(1, 5, 2, 1)| = 1 + 5 + 2 + 1 = 9$ ), so that  $(1, 5, 2, 1) \in \text{Comp}_9$ , or, in other words,  $(1, 5, 2, 1) \models 9$ . Note that the empty composition  $\emptyset$  is a composition of 0. In other words,  $\emptyset \in \text{Comp}_0$ .

For any  $n \in \mathbb{Z}$ , we let  $[n]$  denote the set  $\{1, 2, \dots, n\}$ . This set is empty whenever  $n \leq 0$ , and otherwise has size  $n$ .

If  $X$  is any set, then  $\mathcal{P}(X)$  shall denote the *powerset* of  $X$ . This is the set of all subsets of  $X$ .

## 2. The maps $D$ and $\text{comp}$

It is well-known that any positive integer  $n$  has exactly  $2^{n-1}$  compositions. This has a standard bijective proof ("stars and bars") which relies on the following bijections:

**Definition 2.1.** Let  $n \in \mathbb{N}$ .

(a) We define a map  $D : \text{Comp}_n \rightarrow \mathcal{P}([n-1])$  by setting<sup>1</sup>

$$\begin{aligned} D(\alpha_1, \alpha_2, \dots, \alpha_k) &= \{\alpha_1 + \alpha_2 + \dots + \alpha_i \mid i \in [k-1]\} \\ &= \{\alpha_1, \alpha_1 + \alpha_2, \alpha_1 + \alpha_2 + \alpha_3, \dots, \alpha_1 + \alpha_2 + \dots + \alpha_{k-1}\} \end{aligned}$$

for each  $(\alpha_1, \alpha_2, \dots, \alpha_k) \in \text{Comp}_n$ . (It is easy to see that this map  $D$  is well-defined; see [Grinbe15, detailed version, Lemma 10.4] for a detailed proof.)

(b) We define a map  $\text{comp} : \mathcal{P}([n-1]) \rightarrow \text{Comp}_n$  as follows: For any  $I \in \mathcal{P}([n-1])$ , we set

$$\text{comp}(I) = (i_1 - i_0, i_2 - i_1, \dots, i_m - i_{m-1}),$$

where  $i_0, i_1, \dots, i_m$  are the elements of the set  $I \cup \{0, n\}$  listed in increasing order (so that  $i_0 < i_1 < \dots < i_m$ , therefore  $i_0 = 0$  and  $i_m = n$  and  $\{i_1, i_2, \dots, i_{m-1}\} = I$ ). (It is easy to see that this map  $\text{comp}$  is well-defined; see [Grinbe15, detailed version, Lemma 10.15 (d)] for a detailed proof.)

The maps  $D$  and  $\text{comp}$  are mutually inverse bijections. (See [Grinbe15, detailed version, Proposition 10.17] for a detailed proof of this.)

We note that both of these maps  $D$  and  $\text{comp}$  depend on  $n$ . Thus, they should be denoted by  $D_n$  or  $\text{comp}_n$  to avoid ambiguity. Otherwise, for example, the expression “ $\text{comp}(\{2,3\})$ ” would have different meanings depending on whether  $n$  is 4 or 5. However, we shall not use the map  $\text{comp}$  in what follows. As for the map  $D$ , we need not be afraid of any ambiguity, since the value of  $D(\alpha)$  for a given composition  $\alpha$  is uniquely determined (indeed, the expression “ $D(\alpha)$ ” makes sense only for one value of  $n$ , namely for  $n = |\alpha|$ ; no other value of  $n$  would satisfy  $\alpha \in \text{Comp}_n$ ). Thus, we shall freely use the notation “ $D(\alpha)$ ” without explicitly specifying  $n$ .

The notation  $D$  we just introduced presumably originates in the word “descent”, but the connection between  $D$  and actual descents is indirect and rather misleading. I prefer to call  $D$  the “partial sum map” (as  $D(\alpha)$  consists of the partial sums of the composition  $\alpha$ ) and its inverse  $\text{comp}$  the “interstitial map” (as  $\text{comp}(I)$  consists of the lengths of the intervals into which the elements of  $I$  split the interval  $[n]$ ).

**Example 2.2.** Let  $n = 10$ .

(a) The map  $D$  defined in Definition 2.1 (a) satisfies

$$\begin{aligned} D(1,4,2,3) &= \{1, 1+4, 1+4+2\} = \{1,5,7\}; \\ D(3,5,2) &= \{3, 3+5\} = \{3,8\}; \\ D(1,1,1,1,1,1,1,1,1) &= \{1,2,3,4,5,6,7,8,9\} = [9] = [n-1]; \\ D(10) &= \{\} = \emptyset. \end{aligned}$$

(b) The map  $\text{comp}$  defined in Definition 2.1 (b) satisfies

$$\text{comp}(\{2,3,7\}) = (2-0, 3-2, 7-3, 10-7) = (2,1,4,3)$$

(since  $0,2,3,7,10$  are the elements of the set  $\{2,3,7\} \cup \{0,10\}$  listed in increasing order).

Our first observation about the bijections  $D$  and  $\text{comp}$  concerns the relation between the size of  $D(\alpha)$  and the length  $\ell(\alpha)$  of  $\alpha$ . Namely, we shall show that every composition  $\alpha$  of size  $|\alpha| > 0$  satisfies  $|D(\alpha)| = \ell(\alpha) - 1$ :

**Proposition 2.3.** Let  $\alpha$  be a composition such that  $|\alpha| > 0$ . Then,  $|D(\alpha)| = \ell(\alpha) - 1$ .

Note that the “ $|\alpha| > 0$ ” assumption in Proposition 2.3 is necessary, since Proposition 2.3 would fail if  $\alpha$  was the empty composition  $\emptyset = ()$  (because  $D(\emptyset) = \emptyset$  and thus  $|D(\emptyset)| = 0 \neq \ell(\emptyset) - 1$ ).

---

<sup>1</sup>The notation “ $D(\alpha_1, \alpha_2, \dots, \alpha_k)$ ” means  $D((\alpha_1, \alpha_2, \dots, \alpha_k))$  (that is, the image of the composition  $(\alpha_1, \alpha_2, \dots, \alpha_k)$  under the map  $D$ ).

*Proof of Proposition 2.3.* Write the composition  $\alpha$  in the form  $\alpha = (\alpha_1, \alpha_2, \dots, \alpha_k)$ . Then,  $\ell(\alpha) = k$  (by the definition of  $\ell(\alpha)$ ) and  $|\alpha| = \alpha_1 + \alpha_2 + \dots + \alpha_k$  (by the definition of  $|\alpha|$ ). If we had  $k = 0$ , then we would have

$$\begin{aligned} |\alpha| &= \alpha_1 + \alpha_2 + \dots + \alpha_k = \alpha_1 + \alpha_2 + \dots + \alpha_0 \quad (\text{since } k = 0) \\ &= (\text{empty sum}) = 0, \end{aligned}$$

which would contradict  $|\alpha| > 0$ . Thus, we cannot have  $k = 0$ . Hence,  $k \neq 0$ , so that  $k \geq 1$  (since  $k \in \mathbb{N}$ ).

From  $\alpha = (\alpha_1, \alpha_2, \dots, \alpha_k)$ , we obtain

$$\begin{aligned} D(\alpha) &= D(\alpha_1, \alpha_2, \dots, \alpha_k) \\ &= \{\alpha_1, \alpha_1 + \alpha_2, \alpha_1 + \alpha_2 + \alpha_3, \dots, \alpha_1 + \alpha_2 + \dots + \alpha_{k-1}\} \end{aligned} \quad (1)$$

(by the definition of the map  $D$ ). However, it is easy to see that the chain of inequalities

$$\alpha_1 < \alpha_1 + \alpha_2 < \alpha_1 + \alpha_2 + \alpha_3 < \dots < \alpha_1 + \alpha_2 + \dots + \alpha_{k-1}$$

holds<sup>2</sup>. Thus, the  $k - 1$  numbers  $\alpha_1, \alpha_1 + \alpha_2, \alpha_1 + \alpha_2 + \alpha_3, \dots, \alpha_1 + \alpha_2 + \dots + \alpha_{k-1}$  are distinct. Therefore, the set of these  $k - 1$  numbers has size  $k - 1$ . In other words, we have

$$|\{\alpha_1, \alpha_1 + \alpha_2, \alpha_1 + \alpha_2 + \alpha_3, \dots, \alpha_1 + \alpha_2 + \dots + \alpha_{k-1}\}| = k - 1.$$

In view of (1), we can rewrite this as  $|D(\alpha)| = k - 1$ . In other words,  $|D(\alpha)| = \ell(\alpha) - 1$  (since  $\ell(\alpha) = k$ ). This proves Proposition 2.3.  $\square$

The analogue of Proposition 2.3 for  $|\alpha| = 0$  is almost trivial:

**Proposition 2.4.** Let  $\alpha$  be a composition such that  $|\alpha| = 0$ . Then,  $\alpha = \emptyset$  and  $\ell(\alpha) = 0$  and  $D(\alpha) = \emptyset$ .

---

<sup>2</sup>*Proof.* Let  $i \in [k]$ . Then,  $\alpha_i$  is an entry of  $\alpha$  (since  $\alpha = (\alpha_1, \alpha_2, \dots, \alpha_k)$ ).

Recall that  $\alpha$  is a composition, i.e., a finite list of positive integers. Hence,  $\alpha_i$  is a positive integer (since  $\alpha_i$  is an entry of  $\alpha$ ). Therefore,  $\alpha_i > 0$ . Hence,

$$\alpha_1 + \alpha_2 + \dots + \alpha_i = \alpha_1 + \alpha_2 + \dots + \alpha_{i-1} + \underbrace{\alpha_i}_{>0} > \alpha_1 + \alpha_2 + \dots + \alpha_{i-1}.$$

In other words,  $\alpha_1 + \alpha_2 + \dots + \alpha_{i-1} < \alpha_1 + \alpha_2 + \dots + \alpha_i$ .

Forget that we fixed  $i$ . We thus have proved the inequality  $\alpha_1 + \alpha_2 + \dots + \alpha_{i-1} < \alpha_1 + \alpha_2 + \dots + \alpha_i$  for each  $i \in [k]$ . Hence, in particular, this inequality holds for each  $i \in \{2, 3, \dots, k - 1\}$ . In other words, we have the chain of inequalities

$$\alpha_1 < \alpha_1 + \alpha_2 < \alpha_1 + \alpha_2 + \alpha_3 < \dots < \alpha_1 + \alpha_2 + \dots + \alpha_{k-1}.$$

*Proof of Proposition 2.4.* Write the composition  $\alpha$  in the form  $\alpha = (\alpha_1, \alpha_2, \dots, \alpha_k)$ . Then,  $|\alpha| = \alpha_1 + \alpha_2 + \dots + \alpha_k$  (by the definition of  $|\alpha|$ ) and  $\ell(\alpha) = k$  (by the definition of  $\ell(\alpha)$ ).

Assume (for the sake of contradiction) that  $k \neq 0$ . Thus,  $k \geq 1$  (since  $k \in \mathbb{N}$ ).

However,  $\alpha$  is a composition, i.e., a finite list of positive integers. In other words,  $(\alpha_1, \alpha_2, \dots, \alpha_k)$  is a finite list of positive integers (since  $\alpha = (\alpha_1, \alpha_2, \dots, \alpha_k)$ ). Thus,  $\alpha_1, \alpha_2, \dots, \alpha_k$  are positive integers. Therefore, in particular,  $\alpha_2, \alpha_3, \dots, \alpha_k$  are positive integers. Hence,  $\alpha_2 + \alpha_3 + \dots + \alpha_k \geq 0$  (since a sum of positive integers is always  $\geq 0$ ). However, from  $|\alpha| = 0$ , we obtain

$$\begin{aligned} 0 = |\alpha| &= \alpha_1 + \alpha_2 + \dots + \alpha_k = \alpha_1 + \underbrace{(\alpha_2 + \alpha_3 + \dots + \alpha_k)}_{\geq 0} && (\text{since } k \geq 1) \\ &\geq \alpha_1 > 0 && (\text{since } \alpha_1 \text{ is a positive integer}), \end{aligned}$$

which is absurd. This contradiction shows that our assumption (that  $k \neq 0$ ) was false. Hence,  $k = 0$ .

Now,

$$\begin{aligned} \alpha &= (\alpha_1, \alpha_2, \dots, \alpha_k) = (\alpha_1, \alpha_2, \dots, \alpha_0) && (\text{since } k = 0) \\ &= () = \emptyset && (\text{recall that } \emptyset \text{ denotes the empty composition}). \end{aligned}$$

Moreover,  $\ell(\alpha) = k = 0$ . Finally, from  $\alpha = ()$ , we obtain  $D(\alpha) = D() = \emptyset$  (by the definition of the map  $D : \text{Comp}_0 \rightarrow \mathcal{P}([0-1])$ ). Thus, Proposition 2.4 is proved.  $\square$

We can unite Proposition 2.3 with Proposition 2.4 by using the *Iverson bracket notation*:

**Convention 2.5.** If  $\mathcal{A}$  is a logical statement, then  $[\mathcal{A}]$  shall denote the truth value of  $\mathcal{A}$ ; this is the integer defined by

$$[\mathcal{A}] = \begin{cases} 1, & \text{if } \mathcal{A} \text{ is true;} \\ 0, & \text{if } \mathcal{A} \text{ is false.} \end{cases}$$

For example,  $[2 + 2 = 4] = 1$  (since the statement  $2 + 2 = 4$  is true) and  $[2 + 2 = 5] = 0$  (since the statement  $2 + 2 = 5$  is false).

Now, Proposition 2.3 with Proposition 2.4 can be combined into the following:

**Corollary 2.6.** Let  $n \in \mathbb{N}$ . Let  $\alpha \in \text{Comp}_n$ . Then,  $\ell(\alpha) = |D(\alpha)| + [n \neq 0]$ .

*Proof of Corollary 2.6.* From  $\alpha \in \text{Comp}_n$ , we see that  $\alpha$  is a composition of  $n$  (since  $\text{Comp}_n$  is the set of all compositions of  $n$ ). In other words,  $\alpha$  is a composition having size  $n$ . Therefore,  $|\alpha| = n$  (since  $|\alpha|$  is the size of  $\alpha$ , but we know that  $\alpha$  has size  $n$ ).

We are in one of the following two cases:

Case 1: We have  $n = 0$ .

Case 2: We have  $n \neq 0$ .

Let us first consider Case 1. In this case, we have  $n = 0$ . Hence, we don't have  $n \neq 0$ . Thus,  $[n \neq 0] = 0$ .

However,  $|\alpha| = n = 0$ . Thus, Proposition 2.4 yields  $\alpha = \emptyset$  and  $\ell(\alpha) = 0$  and  $D(\alpha) = \emptyset$ . From  $D(\alpha) = \emptyset$ , we obtain  $|D(\alpha)| = |\emptyset| = 0$ . Thus,  $\underbrace{|D(\alpha)|}_{=0} + \underbrace{[n \neq 0]}_{=0} = 0$ . Comparing this with  $\ell(\alpha) = 0$ , we obtain  $\ell(\alpha) = |D(\alpha)| + [n \neq 0]$ . Hence, Corollary 2.6 is proved in Case 1.

Let us now consider Case 2. In this case, we have  $n \neq 0$ . Hence,  $[n \neq 0] = 1$ . Also, from  $n \neq 0$ , we obtain  $n > 0$  (since  $n \in \mathbb{N}$ ). Thus,  $|\alpha| = n > 0$ . Hence, Proposition 2.3 yields  $|D(\alpha)| = \ell(\alpha) - 1$ . Hence,  $\ell(\alpha) = |D(\alpha)| + 1$ . Comparing this with  $|D(\alpha)| + \underbrace{[n \neq 0]}_{=1} = |D(\alpha)| + 1$ , we obtain  $\ell(\alpha) = |D(\alpha)| + [n \neq 0]$ . Thus,

Corollary 2.6 is proved in Case 2.

We have now proved Corollary 2.6 in both Cases 1 and 2. Hence, Corollary 2.6 always holds.  $\square$

**Corollary 2.7.** Let  $n \in \mathbb{N}$ . Let  $\alpha \in \text{Comp}_n$  and  $\beta \in \text{Comp}_n$ . Then,  $\ell(\beta) - \ell(\alpha) = |D(\beta)| - |D(\alpha)|$ .

*Proof of Corollary 2.7.* Corollary 2.6 yields  $\ell(\alpha) = |D(\alpha)| + [n \neq 0]$ . Corollary 2.6 (applied to  $\beta$  instead of  $\alpha$ ) yields  $\ell(\beta) = |D(\beta)| + [n \neq 0]$ . Hence,

$$\begin{aligned} \underbrace{\ell(\beta)}_{=|D(\beta)|+[n \neq 0]} - \underbrace{\ell(\alpha)}_{=|D(\alpha)|+[n \neq 0]} &= (|D(\beta)| + [n \neq 0]) - (|D(\alpha)| + [n \neq 0]) \\ &= |D(\beta)| - |D(\alpha)|. \end{aligned}$$

This proves Corollary 2.7.  $\square$

### 3. Reversals

We shall now discuss a certain operation on compositions:

**Definition 3.1.** If  $\alpha = (\alpha_1, \alpha_2, \dots, \alpha_k)$  is a composition, then the *reversal* of  $\alpha$  is defined to be the composition  $(\alpha_k, \alpha_{k-1}, \dots, \alpha_1)$ . It is denoted by  $\text{rev } \alpha$ .

Thus, we have defined a map  $\text{rev} : \text{Comp} \rightarrow \text{Comp}$  that sends each composition  $\alpha$  to the composition  $\text{rev } \alpha$ .

**Example 3.2.** We have

$$\begin{aligned} \text{rev}(2, 3, 6) &= (6, 3, 2); \\ \text{rev}(4, 1, 1, 2) &= (2, 1, 1, 4); \\ \text{rev } \emptyset &= \emptyset. \end{aligned}$$

**Proposition 3.3.** Let  $\alpha \in \text{Comp}$ . Then,  $|\text{rev } \alpha| = |\alpha|$ .

*Proof of Proposition 3.3.* Write the composition  $\alpha$  in the form  $\alpha = (\alpha_1, \alpha_2, \dots, \alpha_k)$ . Then,  $\text{rev } \alpha = (\alpha_k, \alpha_{k-1}, \dots, \alpha_1)$  (by Definition 3.1) and  $|\alpha| = \alpha_1 + \alpha_2 + \dots + \alpha_k$  (by the definition of  $|\alpha|$ ). Now,

$$\begin{aligned} |\text{rev } \alpha| &= |(\alpha_k, \alpha_{k-1}, \dots, \alpha_1)| && (\text{since } \text{rev } \alpha = (\alpha_k, \alpha_{k-1}, \dots, \alpha_1)) \\ &= \alpha_k + \alpha_{k-1} + \dots + \alpha_1 && (\text{by the definition of } |(\alpha_k, \alpha_{k-1}, \dots, \alpha_1)|) \\ &= \alpha_1 + \alpha_2 + \dots + \alpha_k \\ &= |\alpha| && (\text{since } |\alpha| = \alpha_1 + \alpha_2 + \dots + \alpha_k). \end{aligned}$$

This proves Proposition 3.3. □

**Proposition 3.4.** Let  $\alpha \in \text{Comp}$ . Then,  $\text{rev}(\text{rev } \alpha) = \alpha$ .

*Proof of Proposition 3.4.* Write the composition  $\alpha$  in the form  $\alpha = (\alpha_1, \alpha_2, \dots, \alpha_k)$ . Then, Definition 3.1 yields  $\text{rev } \alpha = (\alpha_k, \alpha_{k-1}, \dots, \alpha_1)$ . However, Definition 3.1 also yields  $\text{rev}(\alpha_k, \alpha_{k-1}, \dots, \alpha_1) = (\alpha_1, \alpha_2, \dots, \alpha_k)$ . Now,

$$\begin{aligned} \text{rev} \underbrace{(\text{rev } \alpha)}_{=(\alpha_k, \alpha_{k-1}, \dots, \alpha_1)} &= \text{rev}(\alpha_k, \alpha_{k-1}, \dots, \alpha_1) = (\alpha_1, \alpha_2, \dots, \alpha_k) = \alpha. \end{aligned}$$

This proves Proposition 3.4. □

**Corollary 3.5.** The map

$$\begin{aligned} \text{Comp} &\rightarrow \text{Comp}, \\ \delta &\mapsto \text{rev } \delta \end{aligned}$$

is a bijection.

*Proof of Corollary 3.5.* Let us denote this map by  $\text{rev}$  (since the image of any  $\delta \in \text{Comp}$  under this map is already being called  $\text{rev } \delta$ ). Thus, we must prove that this map  $\text{rev}$  is a bijection.

But this is easy: Every  $\alpha \in \text{Comp}$  satisfies

$$\begin{aligned} (\text{rev} \circ \text{rev})(\alpha) &= \text{rev}(\text{rev } \alpha) = \alpha && (\text{by Proposition 3.4}) \\ &= \text{id}(\alpha). \end{aligned}$$

Thus,  $\text{rev} \circ \text{rev} = \text{id}$ . Hence, the map  $\text{rev}$  is inverse to itself. Thus, the map  $\text{rev}$  is invertible, i.e., bijective. In other words, it is a bijection. This proves Corollary 3.5. □

We also define a related operation on subsets of  $[n - 1]$ :

**Definition 3.6.** Let  $n \in \mathbb{N}$ . For any subset  $X$  of  $[n - 1]$ , we let  $\text{rev}_n X$  denote the set  $\{n - x \mid x \in X\}$ .

**Example 3.7.** If  $n = 7$ , then

$$\begin{aligned}\text{rev}_n(\{2, 4\}) &= \{7 - 2, 7 - 4\} = \{5, 3\} = \{3, 5\}; \\ \text{rev}_n(\{1, 2, 5, 6\}) &= \{7 - 1, 7 - 2, 7 - 5, 7 - 6\} = \{6, 5, 2, 1\} = \{1, 2, 5, 6\}; \\ \text{rev}_n(\emptyset) &= \emptyset; \\ \text{rev}_n([6]) &= [6].\end{aligned}$$

Informally speaking, the set  $\text{rev}_n X$  defined in Definition 3.6 is the reflection of the set  $X$  across the midpoint of the interval  $[n - 1]$  (where we regard numbers as points on the number line). From this point of view, all claims of the following theorem are visually obvious:

**Theorem 3.8.** Let  $n \in \mathbb{N}$ . Then:

- (a) We have  $\text{rev}_n X \subseteq [n - 1]$  for each subset  $X$  of  $[n - 1]$ .
- (b) We have  $\text{rev}_n(\text{rev}_n X) = X$  for any subset  $X$  of  $[n - 1]$ .
- (c) If two subsets  $X$  and  $Y$  of  $[n - 1]$  satisfy  $X \subseteq Y$ , then  $\text{rev}_n X \subseteq \text{rev}_n Y$ .
- (d) We have  $|\text{rev}_n X| = |X|$  for any subset  $X$  of  $[n - 1]$ .
- (e) We have  $\text{rev}_n X = \{i \in [n - 1] \mid n - i \in X\}$  for any subset  $X$  of  $[n - 1]$ .
- (f) We have  $\text{rev}_n(X \setminus Y) = (\text{rev}_n X) \setminus (\text{rev}_n Y)$  for any subsets  $X$  and  $Y$  of  $[n - 1]$ .
- (g) We have  $\text{rev}_n(X \cap Y) = (\text{rev}_n X) \cap (\text{rev}_n Y)$  for any subsets  $X$  and  $Y$  of  $[n - 1]$ .
- (h) We have  $\text{rev}_n([n - 1]) = [n - 1]$ .
- (i) We have  $D(\text{rev } \alpha) = \text{rev}_n(D(\alpha))$  for any composition  $\alpha \in \text{Comp}_n$ .

*Proof of Theorem 3.8.* (a) Let  $X$  be a subset of  $[n - 1]$ . Then,  $n - x \in [n - 1]$  for each  $x \in X$ <sup>3</sup>. In other words,

$$\{n - x \mid x \in X\} \subseteq [n - 1].$$

<sup>3</sup>*Proof.* Let  $x \in X$ . Then,  $x \in X \subseteq [n - 1] = \{1, 2, \dots, n - 1\}$ , so that  $n - x \in \{1, 2, \dots, n - 1\} = [n - 1]$ .

Forget that we fixed  $x$ . We thus have shown that  $n - x \in [n - 1]$  for each  $x \in X$ .



This rewrites as  $\text{rev}_n X \subseteq [n-1]$  (since  $\text{rev}_n X$  is defined to be  $\{n-x \mid x \in X\}$ ). This proves Theorem 3.8 (a).

**(b)** Let  $X$  be a subset of  $[n-1]$ . Let  $Y = \text{rev}_n X$ .

Let  $p \in \text{rev}_n Y$ . We shall show that  $p \in X$ .

We have

$$\begin{aligned} p \in \text{rev}_n Y &= \{n-x \mid x \in Y\} && \text{(by the definition of } \text{rev}_n Y) \\ &= \{n-y \mid y \in Y\} && \text{(here, we have renamed the index } x \text{ as } y). \end{aligned}$$

In other words,  $p = n-y$  for some  $y \in Y$ . Consider this  $y$ . Now,

$$y \in Y = \text{rev}_n X = \{n-x \mid x \in X\} \quad \text{(by the definition of } \text{rev}_n X).$$

In other words,  $y = n-x$  for some  $x \in X$ . Consider this  $x$ . Now,  $p = n - \underbrace{y}_{=n-x} = n - (n-x) = x \in X$ .

Forget that we fixed  $p$ . We thus have shown that  $p \in X$  for each  $p \in \text{rev}_n Y$ . In other words,  $\text{rev}_n Y \subseteq X$ .

On the other hand, let  $q \in X$ . Then,  $n-q$  has the form  $n-x$  for some  $x \in X$  (namely, for  $x=q$ ). In other words,  $n-q \in \{n-x \mid x \in X\}$ . Since  $Y = \text{rev}_n X = \{n-x \mid x \in X\}$  (by the definition of  $\text{rev}_n X$ ), we can rewrite this as  $n-q \in Y$ .

Furthermore,  $q = n - (n-q)$ . Hence,  $q$  has the form  $n-x$  for some  $x \in Y$  (namely, for  $x=n-q$ ). In other words,  $q \in \{n-x \mid x \in Y\}$ . Since  $\text{rev}_n Y = \{n-x \mid x \in Y\}$  (by the definition of  $\text{rev}_n Y$ ), we can rewrite this as  $q \in \text{rev}_n Y$ .

Forget that we fixed  $q$ . We thus have shown that  $q \in \text{rev}_n Y$  for each  $q \in X$ . In other words,  $X \subseteq \text{rev}_n Y$ .

Combining this with  $\text{rev}_n Y \subseteq X$ , we obtain  $\text{rev}_n Y = X$ . In other words,  $\text{rev}_n(\text{rev}_n X) = X$  (since  $Y = \text{rev}_n X$ ). This proves Theorem 3.8 (b).

**(c)** Let  $X$  and  $Y$  be two subsets of  $[n-1]$  that satisfy  $X \subseteq Y$ . The definition of  $\text{rev}_n Y$  yields  $\text{rev}_n Y = \{n-x \mid x \in Y\}$ .

Let  $p \in \text{rev}_n X$ . Then,  $p \in \text{rev}_n X = \{n-x \mid x \in X\}$  (by the definition of  $\text{rev}_n X$ ). In other words,  $p = n-x$  for some  $x \in X$ . Consider this  $x$ , and denote it by  $z$ . Thus,  $z \in X$  and  $p = n-z$ .

Now,  $z \in X \subseteq Y$  and  $p = n-z$ . Therefore,  $p = n-x$  for some  $x \in Y$  (namely, for  $x=z$ ). In other words,  $p \in \{n-x \mid x \in Y\}$ . This rewrites as  $p \in \text{rev}_n Y$  (since  $\text{rev}_n Y = \{n-x \mid x \in Y\}$ ).

Forget that we fixed  $p$ . We thus have shown that  $p \in \text{rev}_n Y$  for each  $p \in \text{rev}_n X$ . In other words,  $\text{rev}_n X \subseteq \text{rev}_n Y$ . This proves Theorem 3.8 (c).

**(d)** Let  $X$  be a subset of  $[n-1]$ . Let  $Y = \text{rev}_n X$ .

The definition of  $\text{rev}_n X$  yields  $\text{rev}_n X = \{n-x \mid x \in X\}$ . Thus, the elements of  $\text{rev}_n X$  are precisely the numbers  $n-x$  for  $x \in X$ . Clearly, there are at most  $|X|$  many such numbers (since there are  $|X|$  many elements  $x \in X$ ). Hence, the set  $\text{rev}_n X$  has at most  $|X|$  many elements. In other words,  $|\text{rev}_n X| \leq |X|$ .

The same argument (applied to  $Y$  instead of  $X$ ) yields  $|\text{rev}_n Y| \leq |Y|$ . However, from  $Y = \text{rev}_n X$ , we obtain  $\text{rev}_n Y = \text{rev}_n(\text{rev}_n X) = X$  (by Theorem 3.8 (b)). In view of this, we can rewrite  $|\text{rev}_n Y| \leq |Y|$  as  $|X| \leq |Y|$ .

But from  $Y = \text{rev}_n X$ , we also obtain  $|Y| = |\text{rev}_n X| \leq |X|$ . Combining this inequality with  $|X| \leq |Y|$ , we find  $|X| = |Y| = |\text{rev}_n X|$ . In other words,  $|\text{rev}_n X| = |X|$ . This proves Theorem 3.8 (d).

(e) Let  $X$  be a subset of  $[n-1]$ . Let  $Y = \{i \in [n-1] \mid n-i \in X\}$ . We shall show that  $\text{rev}_n X = Y$ .

Note that  $\text{rev}_n X = \{n-x \mid x \in X\}$  (by the definition of  $\text{rev}_n X$ ).

Let  $p \in \text{rev}_n X$ . Then,  $p \in \text{rev}_n X = \{n-x \mid x \in X\}$ . In other words,  $p = n-x$  for some  $x \in X$ . Consider this  $x$ . Thus,  $p = n-x$ , so that  $n = p+x$ . Therefore,  $n-p = x \in X$ . Also,  $p \in \text{rev}_n X \subseteq [n-1]$  (by Theorem 3.8 (a)). Hence,  $p$  is an element  $i$  of  $[n-1]$  satisfying  $n-i \in X$  (since  $n-p \in X$ ). In other words,  $p \in \{i \in [n-1] \mid n-i \in X\}$ . In other words,  $p \in Y$  (since  $Y = \{i \in [n-1] \mid n-i \in X\}$ ).

Forget that we fixed  $p$ . We thus have shown that  $p \in Y$  for each  $p \in \text{rev}_n X$ . In other words,  $\text{rev}_n X \subseteq Y$ .

Now, let  $q \in Y$ . Thus,  $q \in Y = \{i \in [n-1] \mid n-i \in X\}$ . In other words,  $q$  is an  $i \in [n-1]$  satisfying  $n-i \in X$ . In other words,  $q \in [n-1]$  and  $n-q \in X$ . Furthermore,  $q = n-(n-q)$ . Hence,  $q$  has the form  $n-x$  for some  $x \in X$  (namely, for  $x = n-q$ ). In other words,  $q \in \{n-x \mid x \in X\}$ . This rewrites as  $q \in \text{rev}_n X$  (since  $\text{rev}_n X = \{n-x \mid x \in X\}$ ).

Forget that we fixed  $q$ . We thus have shown that  $q \in \text{rev}_n X$  for each  $q \in Y$ . In other words,  $Y \subseteq \text{rev}_n X$ .

Combining this with  $\text{rev}_n X \subseteq Y$ , we obtain  $\text{rev}_n X = Y = \{i \in [n-1] \mid n-i \in X\}$ . This proves Theorem 3.8 (e).

(f) Let  $X$  and  $Y$  be two subsets of  $[n-1]$ . Then,  $X \setminus Y$  is a subset of  $[n-1]$  as well (since  $X \setminus Y \subseteq X \subseteq [n-1]$ ). Thus,  $\text{rev}_n(X \setminus Y) \subseteq [n-1]$  (by Theorem 3.8 (a), applied to  $X \setminus Y$  instead of  $X$ ). Also,  $(\text{rev}_n X) \setminus (\text{rev}_n Y) \subseteq \text{rev}_n X \subseteq [n-1]$  (by Theorem 3.8 (a)).

Theorem 3.8 (e) yields

$$\text{rev}_n X = \{i \in [n-1] \mid n-i \in X\}.$$

Hence, for any  $i \in [n-1]$ , we have the logical equivalence

$$(i \in \text{rev}_n X) \iff (n-i \in X). \quad (2)$$

The same argument (applied to  $Y$  instead of  $X$ ) shows that for any  $i \in [n-1]$ , we have the logical equivalence

$$(i \in \text{rev}_n Y) \iff (n-i \in Y). \quad (3)$$

The same argument (applied to  $X \setminus Y$  instead of  $Y$ ) shows that for any  $i \in [n-1]$ , we have the logical equivalence

$$(i \in \text{rev}_n(X \setminus Y)) \iff (n-i \in X \setminus Y). \quad (4)$$

Now, for each  $i \in [n - 1]$ , we have the following chain of logical equivalences:

$$\begin{aligned}
 (i \in \text{rev}_n(X \setminus Y)) &\iff (n - i \in X \setminus Y) && \text{(by (4))} \\
 &\iff (n - i \in X \text{ and } n - i \notin Y) \\
 &\iff \left( \underbrace{n - i \in X}_{\substack{\iff (i \in \text{rev}_n X) \\ \text{(by (2))}}} \text{ but not } \underbrace{n - i \in Y}_{\substack{\iff (i \in \text{rev}_n Y) \\ \text{(by (3))}}} \right) \\
 &\iff (i \in \text{rev}_n X \text{ but not } i \in \text{rev}_n Y) \\
 &\iff (i \in \text{rev}_n X \text{ and } i \notin \text{rev}_n Y) \\
 &\iff (i \in (\text{rev}_n X) \setminus (\text{rev}_n Y)). && (5)
 \end{aligned}$$

Now, from  $\text{rev}_n(X \setminus Y) \subseteq [n - 1]$ , we obtain

$$\begin{aligned}
 \text{rev}_n(X \setminus Y) &= [n - 1] \cap (\text{rev}_n(X \setminus Y)) \\
 &= \left\{ i \in [n - 1] \mid \underbrace{i \in \text{rev}_n(X \setminus Y)}_{\substack{\iff (i \in (\text{rev}_n X) \setminus (\text{rev}_n Y)) \\ \text{(by (5))}}} \right\} \\
 &= \{i \in [n - 1] \mid i \in (\text{rev}_n X) \setminus (\text{rev}_n Y)\}. && (6)
 \end{aligned}$$

However, from  $(\text{rev}_n X) \setminus (\text{rev}_n Y) \subseteq [n - 1]$ , we obtain

$$\begin{aligned}
 (\text{rev}_n X) \setminus (\text{rev}_n Y) &= [n - 1] \cap ((\text{rev}_n X) \setminus (\text{rev}_n Y)) \\
 &= \{i \in [n - 1] \mid i \in (\text{rev}_n X) \setminus (\text{rev}_n Y)\}.
 \end{aligned}$$

Comparing this with (6), we find  $\text{rev}_n(X \setminus Y) = (\text{rev}_n X) \setminus (\text{rev}_n Y)$ . This proves Theorem 3.8 **(f)**.

**(g)** Recall that

$$A \setminus (A \setminus B) = A \cap B \quad (7)$$

for any two sets  $A$  and  $B$ .

Let  $X$  and  $Y$  be two subsets of  $[n - 1]$ . Then,  $X \setminus Y$  is a subset of  $[n - 1]$  as well (since  $X \setminus Y \subseteq X \subseteq [n - 1]$ ). Hence, Theorem 3.8 **(f)** (applied to  $X \setminus Y$  instead of  $Y$ ) yields

$$\begin{aligned}
 \text{rev}_n(X \setminus (X \setminus Y)) &= (\text{rev}_n X) \setminus \underbrace{(\text{rev}_n(X \setminus Y))}_{\substack{= (\text{rev}_n X) \setminus (\text{rev}_n Y) \\ \text{(by Theorem 3.8 (f))}}} \\
 &= (\text{rev}_n X) \setminus ((\text{rev}_n X) \setminus (\text{rev}_n Y)) \\
 &= (\text{rev}_n X) \cap (\text{rev}_n Y) && (8)
 \end{aligned}$$

(by (7), applied to  $A = \text{rev}_n X$  and  $B = \text{rev}_n Y$ ). However,  $X \setminus (X \setminus Y) = X \cap Y$  (by (7), applied to  $A = X$  and  $B = Y$ ). Thus, we can rewrite (8) as  $\text{rev}_n (X \cap Y) = (\text{rev}_n X) \cap (\text{rev}_n Y)$ . This proves Theorem 3.8 (g).

(h) The definition of  $\text{rev}_n ([n-1])$  yields

$$\begin{aligned} \text{rev}_n ([n-1]) &= \{n-x \mid x \in [n-1]\} \\ &= \{n-x \mid x \in \{1, 2, \dots, n-1\}\} && (\text{since } [n-1] = \{1, 2, \dots, n-1\}) \\ &= \{n-1, n-2, \dots, n-(n-1)\} \\ &= \{n-1, n-2, \dots, 1\} \\ &= \{1, 2, \dots, n-1\} = [n-1]. \end{aligned}$$

This proves Theorem 3.8 (h).

(i) Let  $\alpha \in \text{Comp}_n$  be a composition. Write this composition  $\alpha$  in the form  $\alpha = (\alpha_1, \alpha_2, \dots, \alpha_k)$ . Then,  $\text{rev } \alpha = (\alpha_k, \alpha_{k-1}, \dots, \alpha_1)$  (by the definition of  $\text{rev } \alpha$ ). Also, the definition of  $|\alpha|$  yields  $|\alpha| = \alpha_1 + \alpha_2 + \dots + \alpha_k$ .

From  $\alpha \in \text{Comp}_n$ , we see that  $\alpha$  is a composition of  $n$  (since  $\text{Comp}_n$  is the set of all compositions of  $n$ ). In other words,  $\alpha$  is a composition having size  $n$ . Therefore,  $|\alpha| = n$  (since  $|\alpha|$  is the size of  $\alpha$ , but we know that  $\alpha$  has size  $n$ ).

For each  $i \in \{0, 1, \dots, k\}$ , we define two numbers

$$\begin{aligned} u_i &:= \alpha_1 + \alpha_2 + \dots + \alpha_i && \text{and} \\ v_i &:= \alpha_{i+1} + \alpha_{i+2} + \dots + \alpha_k. \end{aligned}$$

Each  $i \in \{0, 1, \dots, k\}$  satisfies

$$\begin{aligned} &\underbrace{u_i}_{=\alpha_1+\alpha_2+\dots+\alpha_i} + \underbrace{v_i}_{=\alpha_{i+1}+\alpha_{i+2}+\dots+\alpha_k} \\ &= (\alpha_1 + \alpha_2 + \dots + \alpha_i) + (\alpha_{i+1} + \alpha_{i+2} + \dots + \alpha_k) \\ &= \alpha_1 + \alpha_2 + \dots + \alpha_k = |\alpha| && (\text{since } |\alpha| = \alpha_1 + \alpha_2 + \dots + \alpha_k) \\ &= n \end{aligned}$$

and therefore

$$v_i = n - u_i. \tag{9}$$

From  $\alpha = (\alpha_1, \alpha_2, \dots, \alpha_k)$ , we obtain

$$\begin{aligned} D(\alpha) &= D(\alpha_1, \alpha_2, \dots, \alpha_k) = \left\{ \underbrace{\alpha_1 + \alpha_2 + \dots + \alpha_i}_{\substack{=u_i \\ (\text{since } u_i \text{ is defined} \\ \text{to be } \alpha_1 + \alpha_2 + \dots + \alpha_i)}} \mid i \in [k-1] \right\} \\ &\quad (\text{by the definition of } D(\alpha_1, \alpha_2, \dots, \alpha_k)) \\ &= \{u_i \mid i \in [k-1]\} = \{u_1, u_2, \dots, u_{k-1}\}. \end{aligned}$$


---

The definition of  $\text{rev}_n(D(\alpha))$  yields

$$\begin{aligned}
 \text{rev}_n(D(\alpha)) &= \{n - x \mid x \in D(\alpha)\} \\
 &= \{n - x \mid x \in \{u_1, u_2, \dots, u_{k-1}\}\} \quad (\text{since } D(\alpha) = \{u_1, u_2, \dots, u_{k-1}\}) \\
 &= \{n - u_1, n - u_2, \dots, n - u_{k-1}\} \\
 &= \left\{ \underbrace{n - u_i}_{\substack{=v_i \\ \text{(by (9))}}} \mid i \in [k-1] \right\} = \{v_i \mid i \in [k-1]\} \\
 &= \{v_1, v_2, \dots, v_{k-1}\}.
 \end{aligned}$$

Comparing this with

$$\begin{aligned}
 D(\text{rev } \alpha) &= D(\alpha_k, \alpha_{k-1}, \dots, \alpha_1) \quad (\text{since } \text{rev } \alpha = (\alpha_k, \alpha_{k-1}, \dots, \alpha_1)) \\
 &= \left\{ \underbrace{\alpha_k + \alpha_{k-1} + \dots + \alpha_{k-i+1}}_{\substack{= \alpha_{k-i+1} + \alpha_{k-i+2} + \dots + \alpha_k \\ = v_{k-i} \\ \text{(since } v_{k-i} \text{ is defined} \\ \text{to be } \alpha_{k-i+1} + \alpha_{k-i+2} + \dots + \alpha_k)}} \mid i \in [k-1] \right\} \\
 &\quad (\text{by the definition of } D(\alpha_k, \alpha_{k-1}, \dots, \alpha_1)) \\
 &= \{v_{k-i} \mid i \in [k-1]\} = \{v_{k-1}, v_{k-2}, \dots, v_{k-(k-1)}\} \\
 &= \{v_{k-1}, v_{k-2}, \dots, v_1\} = \{v_1, v_2, \dots, v_{k-1}\},
 \end{aligned}$$

we obtain  $D(\text{rev } \alpha) = \text{rev}_n(D(\alpha))$ . This proves Theorem 3.8 (i).  $\square$

**Corollary 3.9.** Let  $n \in \mathbb{N}$ , and let  $\alpha \in \text{Comp}_n$ . Then,  $\text{rev}_n(D(\text{rev } \alpha)) = D(\alpha)$ .

*Proof of Corollary 3.9.* We have  $\alpha \in \text{Comp}_n$ . In other words,  $\alpha$  is a composition of  $n$ . That is,  $\alpha$  is a composition having size  $n$ . In other words,  $\alpha \in \text{Comp}$  and  $|\alpha| = n$ . Hence, Proposition 3.3 yields  $|\text{rev } \alpha| = |\alpha| = n$ . In other words, the composition  $\text{rev } \alpha$  has size  $n$ . In other words,  $\text{rev } \alpha$  is a composition of  $n$ . In other words,  $\text{rev } \alpha \in \text{Comp}_n$ . Hence,  $D(\text{rev } \alpha) \in \mathcal{P}([n-1])$  (since  $D$  is a map  $\text{Comp}_n \rightarrow \mathcal{P}([n-1])$ ). In other words,  $D(\text{rev } \alpha)$  is a subset of  $[n-1]$ . Hence,  $\text{rev}_n(D(\text{rev } \alpha))$  is well-defined.

Furthermore,  $D(\alpha) \in \mathcal{P}([n-1])$  (since  $D$  is a map  $\text{Comp}_n \rightarrow \mathcal{P}([n-1])$ ). In other words,  $D(\alpha)$  is a subset of  $[n-1]$ .

Theorem 3.8 (i) yields  $D(\text{rev } \alpha) = \text{rev}_n(D(\alpha))$ . Thus,

$$\text{rev}_n \left( \underbrace{D(\text{rev } \alpha)}_{= \text{rev}_n(D(\alpha))} \right) = \text{rev}_n(\text{rev}_n(D(\alpha))) = D(\alpha)$$

(by Theorem 3.8 (b), applied to  $X = D(\alpha)$ ). This proves Corollary 3.9.  $\square$

**Corollary 3.10.** Let  $n \in \mathbb{N}$ . Then, the map

$$\begin{aligned} \text{Comp}_n &\rightarrow \text{Comp}_n, \\ \delta &\mapsto \text{rev } \delta \end{aligned}$$

is a bijection.

*Proof of Corollary 3.10.* Each  $\delta \in \text{Comp}_n$  satisfies  $\text{rev } \delta \in \text{Comp}_n$ <sup>4</sup>. Hence, the map

$$\begin{aligned} \text{Comp}_n &\rightarrow \text{Comp}_n, \\ \delta &\mapsto \text{rev } \delta \end{aligned}$$

is well-defined. It remains to prove that this map is a bijection.

Let us denote this map by  $\text{rev}$  (since the image of any  $\delta \in \text{Comp}$  under this map is already being called  $\text{rev } \delta$ ). Thus, we must prove that this map  $\text{rev}$  is a bijection.

But this is easy: Every  $\alpha \in \text{Comp}_n$  satisfies

$$\begin{aligned} (\text{rev} \circ \text{rev})(\alpha) &= \text{rev}(\text{rev } \alpha) = \alpha && \text{(by Proposition 3.4)} \\ &= \text{id}(\alpha). \end{aligned}$$

Thus,  $\text{rev} \circ \text{rev} = \text{id}$ . Hence, the map  $\text{rev}$  is inverse to itself. Thus, the map  $\text{rev}$  is invertible, i.e., bijective. In other words, it is a bijection. This proves Corollary 3.10.  $\square$

**Proposition 3.11.** Let  $n \in \mathbb{N}$ . Let  $\alpha \in \text{Comp}_n$  and  $\beta \in \text{Comp}_n$  be arbitrary. Then, we have the logical equivalence

$$(D(\text{rev } \beta) \subseteq D(\text{rev } \alpha)) \iff (D(\beta) \subseteq D(\alpha)).$$

*Proof of Proposition 3.11.* We have  $\alpha \in \text{Comp}_n$  and thus  $D(\alpha) \in \mathcal{P}([n-1])$  (since  $D : \text{Comp}_n \rightarrow \mathcal{P}([n-1])$  is a map). In other words,  $D(\alpha)$  is a subset of  $[n-1]$ . Similarly,  $D(\beta)$  is a subset of  $[n-1]$ .

Theorem 3.8 (i) yields  $D(\text{rev } \alpha) = \text{rev}_n(D(\alpha))$ . Also, Theorem 3.8 (i) (applied to  $\beta$  instead of  $\alpha$ ) yields  $D(\text{rev } \beta) = \text{rev}_n(D(\beta))$ .

Now, if  $D(\beta) \subseteq D(\alpha)$ , then  $\text{rev}_n(D(\beta)) \subseteq \text{rev}_n(D(\alpha))$  (by Theorem 3.8 (c), applied to  $X = D(\beta)$  and  $Y = D(\alpha)$ ) and therefore

$$D(\text{rev } \beta) = \text{rev}_n(D(\beta)) \subseteq \text{rev}_n(D(\alpha)) = D(\text{rev } \alpha)$$

---

<sup>4</sup>*Proof.* Let  $\delta \in \text{Comp}_n$ . Thus,  $\delta$  is a composition of  $n$ . In other words,  $\delta$  is a composition that has size  $n$ . In other words,  $\delta$  is a composition and satisfies  $|\delta| = n$ . Now, Proposition 3.3 (applied to  $\alpha = \delta$ ) yields  $|\text{rev } \delta| = |\delta| = n$ . Hence,  $\text{rev } \delta$  is a composition that has size  $n$  (since it has size  $|\text{rev } \delta| = n$ ). In other words,  $\text{rev } \delta$  is a composition of  $n$ . In other words,  $\text{rev } \delta \in \text{Comp}_n$ . Qed.

(since  $D(\operatorname{rev} \alpha) = \operatorname{rev}_n(D(\alpha))$ ). In other words, the implication

$$(D(\beta) \subseteq D(\alpha)) \implies (D(\operatorname{rev} \beta) \subseteq D(\operatorname{rev} \alpha)) \quad (10)$$

holds.

Proposition 3.4 yields  $\operatorname{rev}(\operatorname{rev} \alpha) = \alpha$ . Similarly,  $\operatorname{rev}(\operatorname{rev} \beta) = \beta$ .

However, Corollary 3.10 says that the map

$$\begin{aligned} \operatorname{Comp}_n &\rightarrow \operatorname{Comp}_n, \\ \delta &\mapsto \operatorname{rev} \delta \end{aligned}$$

is a bijection. Thus, in particular, this map is well-defined. In other words, for any  $\delta \in \operatorname{Comp}_n$ , we have  $\operatorname{rev} \delta \in \operatorname{Comp}_n$ . Applying this to  $\delta = \alpha$ , we obtain  $\operatorname{rev} \alpha \in \operatorname{Comp}_n$  (since  $\alpha \in \operatorname{Comp}_n$ ). Similarly,  $\operatorname{rev} \beta \in \operatorname{Comp}_n$ . Thus, we can apply the implication (10) to  $\operatorname{rev} \alpha$  and  $\operatorname{rev} \beta$  instead of  $\alpha$  and  $\beta$ . Hence, we obtain the implication

$$(D(\operatorname{rev} \beta) \subseteq D(\operatorname{rev} \alpha)) \implies (D(\operatorname{rev}(\operatorname{rev} \beta)) \subseteq D(\operatorname{rev}(\operatorname{rev} \alpha))).$$

In view of  $\operatorname{rev}(\operatorname{rev} \alpha) = \alpha$  and  $\operatorname{rev}(\operatorname{rev} \beta) = \beta$ , we can rewrite this as

$$(D(\operatorname{rev} \beta) \subseteq D(\operatorname{rev} \alpha)) \implies (D(\beta) \subseteq D(\alpha)).$$

Combining this implication with (10), we obtain the logical equivalence

$$(D(\operatorname{rev} \beta) \subseteq D(\operatorname{rev} \alpha)) \iff (D(\beta) \subseteq D(\alpha)).$$

This proves Proposition 3.11. □

## 4. The omega operation

**Proposition 4.1.** Let  $n \in \mathbb{N}$ . Let  $\gamma \in \operatorname{Comp}_n$ . Then, there exists a unique composition  $\delta$  of  $n$  satisfying

$$D(\delta) = [n-1] \setminus D(\operatorname{rev} \gamma).$$

*Proof of Proposition 4.1.* The set  $[n-1] \setminus D(\operatorname{rev} \gamma)$  is clearly a subset of  $[n-1]$ , and thus belongs to  $\mathcal{P}([n-1])$ . Hence, there exists a unique  $\delta \in \operatorname{Comp}_n$  satisfying  $D(\delta) = [n-1] \setminus D(\operatorname{rev} \gamma)$  (since the map  $D : \operatorname{Comp}_n \rightarrow \mathcal{P}([n-1])$  is a bijection). In other words, there exists a unique composition  $\delta$  of  $n$  satisfying  $D(\delta) = [n-1] \setminus D(\operatorname{rev} \gamma)$  (because a composition  $\delta$  of  $n$  is the same as an element  $\delta \in \operatorname{Comp}_n$ ). This proves Proposition 4.1. □

We now define another operation on compositions:

**Definition 4.2.** Let  $n \in \mathbb{N}$ . For any composition  $\gamma \in \text{Comp}_n$ , we let  $\omega(\gamma)$  denote the unique composition  $\delta$  of  $n$  satisfying

$$D(\delta) = [n-1] \setminus D(\text{rev } \gamma).$$

(This  $\omega(\gamma)$  is indeed well-defined, according to Proposition 4.1.)

We observe the following simple properties of these compositions  $\omega(\gamma)$ :

**Proposition 4.3.** Let  $n \in \mathbb{N}$ . Let  $\gamma \in \text{Comp}_n$ . Then:

- (a) We have  $\omega(\gamma) \in \text{Comp}_n$ .
- (b) We have  $D(\omega(\gamma)) = [n-1] \setminus D(\text{rev } \gamma)$ .
- (c) We have  $D(\omega(\gamma)) = [n-1] \setminus \text{rev}_n(D(\gamma))$ .
- (d) We have  $\omega(\omega(\gamma)) = \gamma$ .

*Proof of Proposition 4.3.* We have defined  $\omega(\gamma)$  to be the unique composition  $\delta$  of  $n$  satisfying  $D(\delta) = [n-1] \setminus D(\text{rev } \gamma)$ . Thus,  $\omega(\gamma)$  is a composition of  $n$  and satisfies  $D(\omega(\gamma)) = [n-1] \setminus D(\text{rev } \gamma)$ . This proves Proposition 4.3 (b). Moreover, we have  $\omega(\gamma) \in \text{Comp}_n$  (since  $\omega(\gamma)$  is a composition of  $n$ ); this proves Proposition 4.3 (a).

It remains to prove parts (c) and (d).

(c) Theorem 3.8 (i) (applied to  $\alpha = \gamma$ ) yields  $D(\text{rev } \gamma) = \text{rev}_n(D(\gamma))$ . Now,

$$D(\omega(\gamma)) = [n-1] \setminus \underbrace{D(\text{rev } \gamma)}_{=\text{rev}_n(D(\gamma))} = [n-1] \setminus \text{rev}_n(D(\gamma)).$$

This proves Proposition 4.3 (c).

(d) We observe that  $\gamma$  is a composition of  $n$  (since  $\gamma \in \text{Comp}_n$ ). In other words,  $\gamma$  is a composition having size  $n$ . In other words,  $\gamma \in \text{Comp}$  and  $|\gamma| = n$ . However, Proposition 3.3 (applied to  $\alpha = \gamma$ ) yields  $|\text{rev } \gamma| = |\gamma| = n$ . Hence,  $\text{rev } \gamma$  is a composition having size  $|\text{rev } \gamma| = n$ . In other words,  $\text{rev } \gamma$  is a composition of  $n$ . Hence,  $\text{rev } \gamma \in \text{Comp}_n$ . Thus,  $D(\text{rev } \gamma) \in \mathcal{P}([n-1])$  (since  $D$  is a map  $\text{Comp}_n \rightarrow \mathcal{P}([n-1])$ ). In other words,  $D(\text{rev } \gamma)$  is a subset of  $[n-1]$ . Furthermore,  $D(\gamma) \in \mathcal{P}([n-1])$  (since  $\gamma \in \text{Comp}_n$  and since  $D$  is a map  $\text{Comp}_n \rightarrow \mathcal{P}([n-1])$ ). In other words,  $D(\gamma)$  is a subset of  $[n-1]$ . Also,  $[n-1]$  is a subset of  $[n-1]$  as well.



Theorem 3.8 (i) (applied to  $\alpha = \omega(\gamma)$ ) yields

$$\begin{aligned}
 & D(\operatorname{rev}(\omega(\gamma))) \\
 &= \operatorname{rev}_n \left( \underbrace{D(\omega(\gamma))}_{=[n-1] \setminus D(\operatorname{rev} \gamma)} \right) \\
 &= \operatorname{rev}_n([n-1] \setminus D(\operatorname{rev} \gamma)) \\
 &= \underbrace{\operatorname{rev}_n([n-1])}_{=[n-1] \text{ (by Theorem 3.8 (h))}} \setminus \underbrace{\operatorname{rev}_n(D(\operatorname{rev} \gamma))}_{=D(\gamma) \text{ (by Corollary 3.9, applied to } \alpha=\gamma)} \\
 &\quad \text{(by Theorem 3.8 (f), applied to } X=[n-1] \text{ and } Y=D(\operatorname{rev} \gamma)) \\
 &= [n-1] \setminus D(\gamma).
 \end{aligned}$$

We have  $\omega(\omega(\gamma)) \in \operatorname{Comp}_n$  (by Proposition 4.3 (a), applied to  $\omega(\gamma)$  instead of  $\gamma$ ). Moreover, Proposition 4.3 (b) (applied to  $\omega(\gamma)$  instead of  $\gamma$ ) yields

$$\begin{aligned}
 D(\omega(\omega(\gamma))) &= [n-1] \setminus \underbrace{D(\operatorname{rev}(\omega(\gamma)))}_{=[n-1] \setminus D(\gamma)} \\
 &= [n-1] \setminus ([n-1] \setminus D(\gamma)) \\
 &= [n-1] \cap D(\gamma) \quad \left( \begin{array}{l} \text{since } X \setminus (X \setminus Y) = X \cap Y \text{ for} \\ \text{any two sets } X \text{ and } Y \end{array} \right) \\
 &= D(\gamma) \quad (\text{since } D(\gamma) \text{ is a subset of } [n-1]).
 \end{aligned}$$

Recall that the map  $D : \operatorname{Comp}_n \rightarrow \mathcal{P}([n-1])$  is a bijection. Hence, this map is bijective, therefore injective. Thus, any  $\alpha, \beta \in \operatorname{Comp}_n$  satisfying  $D(\alpha) = D(\beta)$  must satisfy  $\alpha = \beta$ . We can apply this to  $\alpha = \omega(\omega(\gamma))$  and  $\beta = \gamma$  (since  $\gamma \in \operatorname{Comp}_n$  and  $\omega(\omega(\gamma)) \in \operatorname{Comp}_n$  and  $D(\omega(\omega(\gamma))) = D(\gamma)$ ), and thus we obtain  $\omega(\omega(\gamma)) = \gamma$ . This proves Proposition 4.3 (d).  $\square$

**Proposition 4.4.** Let  $n$  be a positive integer. Let  $\alpha \in \operatorname{Comp}_n$  and  $\gamma \in \operatorname{Comp}_n$ . Then:

(a) We have

$$|D(\omega(\gamma)) \cap D(\alpha)| = \ell(\alpha) - 1 - |D(\gamma) \cap D(\operatorname{rev} \alpha)|.$$

(b) We have

$$|D(\omega(\gamma)) \setminus D(\alpha)| = n - \ell(\alpha) - |D(\gamma) \setminus D(\operatorname{rev} \alpha)|.$$

*Proof of Proposition 4.4.* We have  $\alpha \in \operatorname{Comp}_n$ . In other words,  $\alpha$  is a composition of  $n$ . That is,  $\alpha$  is a composition having size  $n$ . In other words,  $\alpha \in \operatorname{Comp}$  and  $|\alpha| = n$ . The same argument (applied to  $\gamma$  instead of  $\alpha$ ) yields  $\gamma \in \operatorname{Comp}$  and  $|\gamma| = n$ .

We have  $n \geq 1$  (since  $n$  is a positive integer) and thus  $n - 1 \in \mathbb{N}$ . Hence,  $|[n - 1]| = n - 1$ .

Also, we have  $|\alpha| = n \geq 1 > 0$ . Hence, Proposition 2.3 yields

$$|D(\alpha)| = \ell(\alpha) - 1. \quad (11)$$

Moreover,  $D(\alpha) \in \mathcal{P}([n - 1])$  (since  $D$  is a map  $\text{Comp}_n \rightarrow \mathcal{P}([n - 1])$ ); in other words,  $D(\alpha)$  is a subset of  $[n - 1]$ . The same argument (applied to  $\gamma$  instead of  $\alpha$ ) shows that  $D(\gamma)$  is a subset of  $[n - 1]$ . That is, we have  $D(\gamma) \subseteq [n - 1]$ . Hence,  $\text{rev}_n(D(\gamma)) \subseteq [n - 1]$  as well (by Theorem 3.8 (a), applied to  $X = D(\gamma)$ ).

Also,  $D(\text{rev } \alpha)$  is a subset of  $[n - 1]$  (this can be easily proved in the same way as in the proof of Corollary 3.9 above).

Proposition 4.3 (c) yields  $D(\omega(\gamma)) = [n - 1] \setminus \text{rev}_n(D(\gamma))$ .

However, for any three sets  $X$ ,  $Y$  and  $Z$ , we have  $(X \setminus Y) \cap Z = (X \cap Z) \setminus Y$ . Applying this to  $X = [n - 1]$  and  $Y = \text{rev}_n(D(\gamma))$  and  $Z = D(\alpha)$ , we obtain

$$\begin{aligned} ([n - 1] \setminus \text{rev}_n(D(\gamma))) \cap D(\alpha) &= \underbrace{([n - 1] \cap D(\alpha))}_{\substack{=D(\alpha) \\ \text{(since } D(\alpha) \text{ is a} \\ \text{subset of } [n-1])}} \setminus \text{rev}_n(D(\gamma)) \\ &= D(\alpha) \setminus \text{rev}_n(D(\gamma)). \end{aligned}$$

Thus,

$$\begin{aligned} \underbrace{D(\omega(\gamma))}_{=[n-1] \setminus \text{rev}_n(D(\gamma))} \cap D(\alpha) &= ([n - 1] \setminus \text{rev}_n(D(\gamma))) \cap D(\alpha) \\ &= D(\alpha) \setminus \text{rev}_n(D(\gamma)). \end{aligned}$$

Therefore,

$$\begin{aligned} |D(\omega(\gamma)) \cap D(\alpha)| &= |D(\alpha) \setminus \text{rev}_n(D(\gamma))| \\ &= |D(\alpha)| - |D(\alpha) \cap \text{rev}_n(D(\gamma))| \end{aligned} \quad (12)$$

(since any finite sets  $X$  and  $Y$  satisfy  $|X \setminus Y| = |X| - |X \cap Y|$ ).

However, Theorem 3.8 (g) (applied to  $X = D(\gamma)$  and  $Y = D(\text{rev } \alpha)$ ) yields

$$\begin{aligned} \text{rev}_n(D(\gamma) \cap D(\text{rev } \alpha)) &= \text{rev}_n(D(\gamma)) \cap \underbrace{\text{rev}_n(D(\text{rev } \alpha))}_{\substack{=D(\alpha) \\ \text{(by Corollary 3.9)}}} = \text{rev}_n(D(\gamma)) \cap D(\alpha) \\ &= D(\alpha) \cap \text{rev}_n(D(\gamma)). \end{aligned} \quad (13)$$

However,  $D(\gamma) \cap D(\text{rev } \alpha)$  is a subset of  $[n - 1]$  (since  $D(\gamma) \cap D(\text{rev } \alpha) \subseteq D(\gamma) \subseteq [n - 1]$ ). Hence, Theorem 3.8 (d) (applied to  $X = D(\gamma) \cap D(\text{rev } \alpha)$ ) yields

$$|\text{rev}_n(D(\gamma) \cap D(\text{rev } \alpha))| = |D(\gamma) \cap D(\text{rev } \alpha)|.$$


---

In view of (13), we can rewrite this as

$$|D(\alpha) \cap \text{rev}_n(D(\gamma))| = |D(\gamma) \cap D(\text{rev } \alpha)|.$$

Therefore, (12) becomes

$$\begin{aligned} |D(\omega(\gamma)) \cap D(\alpha)| &= \underbrace{|D(\alpha)|}_{=\ell(\alpha)-1 \text{ (by (11))}} - \underbrace{|D(\alpha) \cap \text{rev}_n(D(\gamma))|}_{=|D(\gamma) \cap D(\text{rev } \alpha)|} \\ &= \ell(\alpha) - 1 - |D(\gamma) \cap D(\text{rev } \alpha)|. \end{aligned}$$

This proves Proposition 4.4 (a).

**(b)** From Proposition 4.3 (c), we obtain  $D(\omega(\gamma)) = [n-1] \setminus \text{rev}_n(D(\gamma))$ .

However, if two finite sets  $X$  and  $Y$  satisfy  $Y \subseteq X$ , then  $|X \setminus Y| = |X| - |Y|$ . Applying this to  $X = [n-1]$  and  $Y = \text{rev}_n(D(\gamma))$ , we obtain

$$\begin{aligned} |[n-1] \setminus \text{rev}_n(D(\gamma))| &= \underbrace{|[n-1]|}_{=n-1} - \underbrace{|\text{rev}_n(D(\gamma))|}_{=|D(\gamma)| \text{ (by Theorem 3.8 (d), applied to } X=D(\gamma))} \quad (\text{since } \text{rev}_n(D(\gamma)) \subseteq [n-1]) \\ &= n-1 - |D(\gamma)|. \end{aligned}$$

In view of  $D(\omega(\gamma)) = [n-1] \setminus \text{rev}_n(D(\gamma))$ , we can rewrite this as

$$|D(\omega(\gamma))| = n-1 - |D(\gamma)|. \quad (14)$$

Next, recall that  $|X \setminus Y| = |X| - |X \cap Y|$  for any two finite sets  $X$  and  $Y$ . From this equality, we obtain

$$|D(\omega(\gamma)) \setminus D(\alpha)| = |D(\omega(\gamma))| - |D(\omega(\gamma)) \cap D(\alpha)| \quad (15)$$

and

$$|D(\gamma) \setminus D(\text{rev } \alpha)| = |D(\gamma)| - |D(\gamma) \cap D(\text{rev } \alpha)|. \quad (16)$$

Adding these two equalities together, we find

$$\begin{aligned} &|D(\omega(\gamma)) \setminus D(\alpha)| + |D(\gamma) \setminus D(\text{rev } \alpha)| \\ &= \underbrace{|D(\omega(\gamma))|}_{=n-1-|D(\gamma)| \text{ (by (14))}} - \underbrace{|D(\omega(\gamma)) \cap D(\alpha)|}_{=\ell(\alpha)-1-|D(\gamma) \cap D(\text{rev } \alpha)| \text{ (by Proposition 4.4 (a))}} + |D(\gamma)| - |D(\gamma) \cap D(\text{rev } \alpha)| \\ &= n-1 - |D(\gamma)| - (\ell(\alpha) - 1 - |D(\gamma) \cap D(\text{rev } \alpha)|) + |D(\gamma)| - |D(\gamma) \cap D(\text{rev } \alpha)| \\ &= n - \ell(\alpha). \end{aligned}$$

In other words,

$$|D(\omega(\gamma)) \setminus D(\alpha)| = n - \ell(\alpha) - |D(\gamma) \setminus D(\text{rev } \alpha)|.$$

This proves Proposition 4.4 (b). □

## 5. Concatenation

### 5.1. Definition and basic properties

The simplest binary operation on compositions is concatenation:

**Definition 5.1.** The *concatenation* of two compositions  $\beta = (\beta_1, \beta_2, \dots, \beta_p)$  and  $\gamma = (\gamma_1, \gamma_2, \dots, \gamma_q)$  is defined to be the composition

$$(\beta_1, \beta_2, \dots, \beta_p, \gamma_1, \gamma_2, \dots, \gamma_q).$$

It is denoted by  $\beta\gamma$ .

It is clear that any composition  $\alpha$  satisfies  $\alpha\emptyset = \emptyset\alpha = \alpha$  (where  $\emptyset$  denotes the empty composition, as before). The next fact is also evident:

**Proposition 5.2.** Let  $\beta$  and  $\gamma$  be two compositions. Then:

- (a) We have  $\ell(\beta\gamma) = \ell(\beta) + \ell(\gamma)$ .
- (b) We have  $|\beta\gamma| = |\beta| + |\gamma|$ .

*Proof of Proposition 5.2.* Write the compositions  $\beta$  and  $\gamma$  in the forms  $\beta = (\beta_1, \beta_2, \dots, \beta_p)$  and  $\gamma = (\gamma_1, \gamma_2, \dots, \gamma_q)$ . Thus, the definition of  $\beta\gamma$  yields

$$\beta\gamma = (\beta_1, \beta_2, \dots, \beta_p, \gamma_1, \gamma_2, \dots, \gamma_q).$$

Hence, the definition of  $\ell(\beta\gamma)$  yields  $\ell(\beta\gamma) = p + q$ , whereas the definition of  $|\beta\gamma|$  yields

$$|\beta\gamma| = \beta_1 + \beta_2 + \dots + \beta_p + \gamma_1 + \gamma_2 + \dots + \gamma_q. \quad (17)$$

However, from  $\beta = (\beta_1, \beta_2, \dots, \beta_p)$ , we obtain  $\ell(\beta) = p$  and  $|\beta| = \beta_1 + \beta_2 + \dots + \beta_p$ . Moreover, from  $\gamma = (\gamma_1, \gamma_2, \dots, \gamma_q)$ , we obtain  $\ell(\gamma) = q$  and  $|\gamma| = \gamma_1 + \gamma_2 + \dots + \gamma_q$ . Thus,

$$\underbrace{\ell(\beta)}_{=p} + \underbrace{\ell(\gamma)}_{=q} = p + q = \ell(\beta\gamma) \quad (\text{since } \ell(\beta\gamma) = p + q).$$

This proves Proposition 5.2 (a).

(b) Adding the equalities  $|\beta| = \beta_1 + \beta_2 + \dots + \beta_p$  and  $|\gamma| = \gamma_1 + \gamma_2 + \dots + \gamma_q$  together, we obtain

$$|\beta| + |\gamma| = \beta_1 + \beta_2 + \dots + \beta_p + \gamma_1 + \gamma_2 + \dots + \gamma_q = |\beta\gamma|$$

(by (17)). This proves Proposition 5.2 (b). □

## 5.2. Concatenation and reversal

Concatenation and reversal interact in a nice way:

**Proposition 5.3.** Let  $\beta$  and  $\gamma$  be two compositions. Then,  $\text{rev}(\beta\gamma) = (\text{rev } \gamma)(\text{rev } \beta)$ .

*Proof of Proposition 5.3.* Write the compositions  $\beta$  and  $\gamma$  in the forms  $\beta = (\beta_1, \beta_2, \dots, \beta_p)$  and  $\gamma = (\gamma_1, \gamma_2, \dots, \gamma_q)$ . Thus, the definition of  $\beta\gamma$  yields

$$\beta\gamma = (\beta_1, \beta_2, \dots, \beta_p, \gamma_1, \gamma_2, \dots, \gamma_q).$$

Hence, the definition of  $\text{rev}(\beta\gamma)$  yields

$$\text{rev}(\beta\gamma) = (\gamma_q, \gamma_{q-1}, \dots, \gamma_1, \beta_p, \beta_{p-1}, \dots, \beta_1). \quad (18)$$

However, the definition of  $\text{rev } \beta$  yields  $\text{rev } \beta = (\beta_p, \beta_{p-1}, \dots, \beta_1)$  (since  $\beta = (\beta_1, \beta_2, \dots, \beta_p)$ ). Furthermore, the definition of  $\text{rev } \gamma$  yields  $\text{rev } \gamma = (\gamma_q, \gamma_{q-1}, \dots, \gamma_1)$  (since  $\gamma = (\gamma_1, \gamma_2, \dots, \gamma_q)$ ). Thus,

$$\begin{aligned} & \underbrace{(\text{rev } \gamma)}_{=(\gamma_q, \gamma_{q-1}, \dots, \gamma_1)} \underbrace{(\text{rev } \beta)}_{=(\beta_p, \beta_{p-1}, \dots, \beta_1)} \\ &= (\gamma_q, \gamma_{q-1}, \dots, \gamma_1) (\beta_p, \beta_{p-1}, \dots, \beta_1) \\ &= (\gamma_q, \gamma_{q-1}, \dots, \gamma_1, \beta_p, \beta_{p-1}, \dots, \beta_1) \end{aligned}$$

(by the definition of concatenation). Comparing this with (18), we obtain  $\text{rev}(\beta\gamma) = (\text{rev } \gamma)(\text{rev } \beta)$ . This proves Proposition 5.3.  $\square$

## 5.3. Concatenation and partial sums

We shall next show some less trivial properties of concatenations of compositions. We will need the following notation:

**Definition 5.4.** If  $K$  is a set of integers, and if  $m$  is an integer, then we define two sets  $K + m$  and  $K - m$  by

$$\begin{aligned} K + m &:= \{k + m \mid k \in K\}, \\ K - m &:= \{k - m \mid k \in K\}. \end{aligned}$$

Clearly, both of these sets  $K + m$  and  $K - m$  are again sets of integers.

For example,  $\{2, 3, 5\} + 10 = \{12, 13, 15\}$  and  $\{2, 3, 5\} - 1 = \{1, 2, 4\}$ . Visually, you can think of  $K + m$  as being the set  $K$ , moved to the right by  $m$  units on the number line. Similarly,  $K - m$  is the set  $K$ , moved to the left by  $m$  units on the number line.

Clearly, if  $K$  is any set of integers, and if  $m$  is an integer, then  $(K + m) - m = K$  and  $(K - m) + m = K$ .

Now, if we know the sizes and the partial sum sets of two compositions  $\beta$  and  $\gamma$ , then we can compute the partial sum set of their concatenation  $\beta\gamma$  as follows:

**Proposition 5.5.** Let  $\beta$  and  $\gamma$  be two compositions such that  $\beta \neq \emptyset$  and  $\gamma \neq \emptyset$ . Let  $m = |\beta|$ . Then,

$$D(\beta\gamma) = \{m\} \cup D(\beta) \cup (D(\gamma) + m).$$

*Proof of Proposition 5.5.* Write the compositions  $\beta$  and  $\gamma$  in the forms  $\beta = (\beta_1, \beta_2, \dots, \beta_p)$  and  $\gamma = (\gamma_1, \gamma_2, \dots, \gamma_q)$ . From  $\beta \neq \emptyset$ , we easily obtain  $p \neq 0$ <sup>5</sup>. Similarly, from  $\gamma \neq \emptyset$ , we obtain  $q \neq 0$ . Also,  $m = |\beta| = \beta_1 + \beta_2 + \dots + \beta_p$  (by the definition of  $|\beta|$ , since  $\beta = (\beta_1, \beta_2, \dots, \beta_p)$ ). Thus,  $\beta_1 + \beta_2 + \dots + \beta_p = m$ .

From  $\beta = (\beta_1, \beta_2, \dots, \beta_p)$ , we obtain

$$D(\beta) = \{\beta_1, \beta_1 + \beta_2, \beta_1 + \beta_2 + \beta_3, \dots, \beta_1 + \beta_2 + \dots + \beta_{p-1}\} \quad (19)$$

(by the definition of  $D(\beta)$ ).

From  $\gamma = (\gamma_1, \gamma_2, \dots, \gamma_q)$ , we obtain

$$D(\gamma) = \{\gamma_1, \gamma_1 + \gamma_2, \gamma_1 + \gamma_2 + \gamma_3, \dots, \gamma_1 + \gamma_2 + \dots + \gamma_{q-1}\}.$$

However, the definition of  $D(\gamma) + m$  yields

$$\begin{aligned} D(\gamma) + m &= \left\{ \underbrace{k + m}_{=m+k} \mid k \in D(\gamma) \right\} = \{m + k \mid k \in D(\gamma)\} \\ &= \{m + k \mid k \in \{\gamma_1, \gamma_1 + \gamma_2, \gamma_1 + \gamma_2 + \gamma_3, \dots, \gamma_1 + \gamma_2 + \dots + \gamma_{q-1}\}\} \\ &\quad (\text{since } D(\gamma) = \{\gamma_1, \gamma_1 + \gamma_2, \gamma_1 + \gamma_2 + \gamma_3, \dots, \gamma_1 + \gamma_2 + \dots + \gamma_{q-1}\}) \\ &= \{m + \gamma_1, m + \gamma_1 + \gamma_2, m + \gamma_1 + \gamma_2 + \gamma_3, \dots, m + \gamma_1 + \gamma_2 + \dots + \gamma_{q-1}\}. \end{aligned} \quad (20)$$

Now, recall that  $\beta = (\beta_1, \beta_2, \dots, \beta_p)$  and  $\gamma = (\gamma_1, \gamma_2, \dots, \gamma_q)$ . Hence, the definition of  $\beta\gamma$  yields

$$\beta\gamma = (\beta_1, \beta_2, \dots, \beta_p, \gamma_1, \gamma_2, \dots, \gamma_q).$$

---

<sup>5</sup>*Proof.* If we had  $p = 0$ , then we would have

$$\begin{aligned} \beta &= (\beta_1, \beta_2, \dots, \beta_p) = (\beta_1, \beta_2, \dots, \beta_0) \quad (\text{since } p = 0) \\ &= () = \emptyset, \end{aligned}$$

which would contradict  $\beta \neq \emptyset$ . Hence, we cannot have  $p = 0$ . Thus, we have  $p \neq 0$ .

---

Hence, the definition of  $D(\beta\gamma)$  yields<sup>6</sup>

$$\begin{aligned}
& D(\beta\gamma) \\
&= \{\beta_1, \beta_1 + \beta_2, \beta_1 + \beta_2 + \beta_3, \dots, \beta_1 + \beta_2 + \dots + \beta_{p-1}, \\
&\quad \beta_1 + \beta_2 + \dots + \beta_p, \\
&\quad \beta_1 + \beta_2 + \dots + \beta_p + \gamma_1, \\
&\quad \beta_1 + \beta_2 + \dots + \beta_p + \gamma_1 + \gamma_2, \\
&\quad \beta_1 + \beta_2 + \dots + \beta_p + \gamma_1 + \gamma_2 + \gamma_3, \\
&\quad \dots, \\
&\quad \beta_1 + \beta_2 + \dots + \beta_p + \gamma_1 + \gamma_2 + \dots + \gamma_{q-1}\} \\
&= \{\beta_1, \beta_1 + \beta_2, \beta_1 + \beta_2 + \beta_3, \dots, \beta_1 + \beta_2 + \dots + \beta_{p-1}, \\
&\quad m, m + \gamma_1, m + \gamma_1 + \gamma_2, m + \gamma_1 + \gamma_2 + \gamma_3, \dots, m + \gamma_1 + \gamma_2 + \dots + \gamma_{q-1}\} \\
&\quad (\text{since } \beta_1 + \beta_2 + \dots + \beta_p = m) \\
&= \underbrace{\{\beta_1, \beta_1 + \beta_2, \beta_1 + \beta_2 + \beta_3, \dots, \beta_1 + \beta_2 + \dots + \beta_{p-1}\}}_{\substack{=D(\beta) \\ (\text{by (19))}}}} \\
&\quad \cup \{m\} \\
&\quad \cup \underbrace{\{m + \gamma_1, m + \gamma_1 + \gamma_2, m + \gamma_1 + \gamma_2 + \gamma_3, \dots, m + \gamma_1 + \gamma_2 + \dots + \gamma_{q-1}\}}_{\substack{=D(\gamma)+m \\ (\text{by (20))}}} \\
&= D(\beta) \cup \{m\} \cup (D(\gamma) + \{m\}) = \{m\} \cup D(\beta) \cup (D(\gamma) + m).
\end{aligned}$$

This proves Proposition 5.5. □

The following is a variant of Proposition 5.5 that avoids the requirements that  $\beta \neq \emptyset$  and  $\gamma \neq \emptyset$ :

**Proposition 5.6.** Let  $\beta$  and  $\gamma$  be two compositions. Let  $m = |\beta|$  and  $n = |\gamma|$ . Then,

$$D(\beta\gamma) = (\{m\} \cup D(\beta) \cup (D(\gamma) + m)) \cap [m + n - 1].$$

*Proof of Proposition 5.6.* We know that  $\gamma$  is a composition having size  $n$  (since the size of  $\gamma$  is  $|\gamma| = n$ ). In other words,  $\gamma$  is a composition of  $n$ . In other words,  $\gamma \in \text{Comp}_n$  (since  $\text{Comp}_n$  is the set of all compositions of  $n$ ).

We know that  $\beta$  is a composition having size  $m$  (since the size of  $\beta$  is  $|\beta| = m$ ). In other words,  $\beta$  is a composition of  $m$ . In other words,  $\beta \in \text{Comp}_m$  (since  $\text{Comp}_m$  is the set of all compositions of  $m$ ).

We have  $0 \notin [n - 1]$  (since the set  $[n - 1] = \{1, 2, \dots, n - 1\}$  does not contain 0) and  $m \notin [m - 1]$  (since the set  $[m - 1] = \{1, 2, \dots, m - 1\}$  does not contain  $m$ ).

---

<sup>6</sup>Note the tacit use of  $p \neq 0$  and  $q \neq 0$  in this computation.

We are in one of the following three cases:

Case 1: We have  $\beta = \emptyset$ .

Case 2: We have  $\gamma = \emptyset$ .

Case 3: We have neither  $\beta = \emptyset$  nor  $\gamma = \emptyset$ .

Let us first consider Case 1. In this case, we have  $\beta = \emptyset$ . Thus,  $D(\beta) = D(\emptyset) = \emptyset$  (by the definition of the map  $D : \text{Comp}_0 \rightarrow \mathcal{P}([0-1])$ ).

Moreover,  $m = |\beta|$ . In view of  $\beta = \emptyset$ , this rewrites as  $m = |\emptyset| = 0$ . Thus,  $D(\gamma) + \underbrace{m}_{=0} = D(\gamma) + 0 = D(\gamma)$  (because any set  $K$  of integers satisfies  $K + 0 = K$ ).

Recall that  $D$  is a map  $\text{Comp}_n \rightarrow \mathcal{P}([n-1])$ . Hence,  $D(\gamma) \in \mathcal{P}([n-1])$  (since  $\gamma \in \text{Comp}_n$ ). In other words,  $D(\gamma) \subseteq [n-1]$ .

Now,

$$\begin{aligned} & \left( \left\{ \underbrace{m}_{=0} \right\} \cup \underbrace{D(\beta)}_{=\emptyset} \cup \underbrace{(D(\gamma) + m)}_{=D(\gamma)} \right) \cap \left[ \underbrace{m}_{=0} + n - 1 \right] \\ &= \left( \underbrace{\{0\} \cup \emptyset \cup D(\gamma)}_{=\{0\}} \right) \cap \left[ \underbrace{0 + n - 1}_{=n-1} \right] \\ &= (\{0\} \cup D(\gamma)) \cap [n-1]. \end{aligned} \tag{21}$$

However, recall that any three sets  $X_1, X_2, Y$  satisfy

$$(X_1 \cup X_2) \cap Y = (X_1 \cap Y) \cup (X_2 \cap Y).$$

Applying this to  $X_1 = \{0\}$ ,  $X_2 = D(\gamma)$  and  $Y = [n-1]$ , we obtain

$$\begin{aligned} (\{0\} \cup D(\gamma)) \cap [n-1] &= \underbrace{(\{0\} \cap [n-1])}_{=\emptyset \text{ (since } 0 \notin [n-1])} \cup \underbrace{(D(\gamma) \cap [n-1])}_{=D(\gamma) \text{ (since } D(\gamma) \subseteq [n-1])} \\ &= \emptyset \cup D(\gamma) = D(\gamma). \end{aligned}$$

Thus, (21) rewrites as

$$\begin{aligned} & (\{m\} \cup D(\beta) \cup (D(\gamma) + m)) \cap [m + n - 1] \\ &= D(\gamma) = D(\beta\gamma) \quad \left( \text{since } \gamma = \beta\gamma \text{ (because } \underbrace{\beta}_{=\emptyset} \gamma = \emptyset\gamma = \gamma) \right). \end{aligned}$$

Hence, Proposition 5.6 is proved in Case 1.

Let us now consider Case 2. In this case, we have  $\gamma = \emptyset$ . Hence,  $D(\gamma) = D(\emptyset) = \emptyset$ . Hence,  $\underbrace{D(\gamma) + m}_{=\emptyset} = \emptyset + m = \emptyset$  (since  $\emptyset + k = \emptyset$  for any integer  $k$ ).



Moreover,  $n = |\gamma|$ . In view of  $\gamma = \emptyset$ , this rewrites as  $n = |\emptyset| = 0$ .

Recall that  $D$  is a map  $\text{Comp}_m \rightarrow \mathcal{P}([m-1])$ . Hence,  $D(\beta) \in \mathcal{P}([m-1])$  (since  $\beta \in \text{Comp}_m$ ). In other words,  $D(\beta) \subseteq [m-1]$ .

Now,

$$\begin{aligned} & \left( \{m\} \cup D(\beta) \cup \underbrace{(D(\gamma) + m)}_{=\emptyset} \right) \cap \left[ m + \underbrace{n}_{=0} - 1 \right] \\ &= \underbrace{(\{m\} \cup D(\beta) \cup \emptyset)}_{=\{m\} \cup D(\beta)} \cap \left[ \underbrace{m + 0 - 1}_{=m-1} \right] \\ &= (\{m\} \cup D(\beta)) \cap [m-1]. \end{aligned} \tag{22}$$

However, recall that any three sets  $X_1, X_2, Y$  satisfy

$$(X_1 \cup X_2) \cap Y = (X_1 \cap Y) \cup (X_2 \cap Y).$$

Applying this to  $X_1 = \{m\}$ ,  $X_2 = D(\beta)$  and  $Y = [m-1]$ , we obtain

$$\begin{aligned} (\{m\} \cup D(\beta)) \cap [m-1] &= \underbrace{(\{m\} \cap [m-1])}_{=\emptyset \text{ (since } m \notin [m-1])} \cup \underbrace{(D(\beta) \cap [m-1])}_{=D(\beta) \text{ (since } D(\beta) \subseteq [m-1])} \\ &= \emptyset \cup D(\beta) = D(\beta). \end{aligned}$$

Thus, (22) rewrites as

$$\begin{aligned} & (\{m\} \cup D(\beta) \cup (D(\gamma) + m)) \cap [m+n-1] \\ &= D(\beta) = D(\beta\gamma) \quad \left( \text{since } \beta = \beta\gamma \text{ (because } \beta \underbrace{\gamma}_{=\emptyset} = \beta\emptyset = \beta) \right). \end{aligned}$$

Hence, Proposition 5.6 is proved in Case 2.

Now, let us consider Case 3. In this case, we have neither  $\beta = \emptyset$  nor  $\gamma = \emptyset$ . In other words, we have  $\beta \neq \emptyset$  and  $\gamma \neq \emptyset$ . Thus, Proposition 5.5 yields

$$D(\beta\gamma) = \{m\} \cup D(\beta) \cup (D(\gamma) + m).$$

However, Proposition 5.2 (b) yields  $|\beta\gamma| = \underbrace{|\beta|}_{=m} + \underbrace{|\gamma|}_{=n} = m+n$ . Thus, the com-

position  $\beta\gamma$  has size  $|\beta\gamma| = m+n$ . In other words,  $\beta\gamma$  is a composition of  $m+n$ . In other words,  $\beta\gamma \in \text{Comp}_{m+n}$ . Hence,  $D(\beta\gamma) \in \mathcal{P}([m+n-1])$  (since  $D$  is a map  $\text{Comp}_{m+n} \rightarrow \mathcal{P}([m+n-1])$ ). In other words,  $D(\beta\gamma) \subseteq [m+n-1]$ . Hence,  $D(\beta\gamma) \cap [m+n-1] = D(\beta\gamma)$ , so that

$$\begin{aligned} D(\beta\gamma) &= \underbrace{D(\beta\gamma)}_{=\{m\} \cup D(\beta) \cup (D(\gamma) + m)} \cap [m+n-1] \\ &= (\{m\} \cup D(\beta) \cup (D(\gamma) + m)) \cap [m+n-1]. \end{aligned}$$

Therefore, Proposition 5.6 is proved in Case 3.

We have now proved Proposition 5.6 in each of the three Cases 1, 2 and 3. This completes the proof of Proposition 5.6.  $\square$

Conversely, given two compositions  $\beta$  and  $\gamma$ , we can reconstruct the partial sum sets  $D(\beta)$  and  $D(\gamma)$  if we know the size  $|\beta|$  and the partial sum set  $D(\beta\gamma)$  as follows:

**Proposition 5.7.** Let  $\beta$  and  $\gamma$  be two compositions. Let  $m = |\beta|$ . Then:

- (a) We have  $D(\beta) = D(\beta\gamma) \cap [m-1]$ .
- (b) We have  $D(\gamma) = (D(\beta\gamma) \setminus [m]) - m$ .

*Proof of Proposition 5.7.* Let  $n = |\gamma|$ . Then, as in the above proof of Proposition 5.6, we can show that  $\beta \in \text{Comp}_m$  and  $\gamma \in \text{Comp}_n$ .

Recall that  $D$  is a map  $\text{Comp}_n \rightarrow \mathcal{P}([n-1])$ . Hence,  $D(\gamma) \in \mathcal{P}([n-1])$  (since  $\gamma \in \text{Comp}_n$ ). In other words,  $D(\gamma) \subseteq [n-1]$ . The same argument (applied to  $\beta$  and  $m$  instead of  $\gamma$  and  $n$ ) yields  $D(\beta) \subseteq [m-1]$ . Also, note that  $[m-1] \subseteq [m+n-1]$  (since  $m-1 \leq m+n-1$  (because  $n \geq 0$ )).

(a) Let  $x \in D(\beta)$ . We shall show that  $x \in D(\beta\gamma) \cap [m-1]$ .

Indeed, we observe that

$$x \in D(\beta) \subseteq \{m\} \cup D(\beta) \cup (D(\gamma) + m).$$

Combining this with  $x \in D(\beta) \subseteq [m-1] \subseteq [m+n-1]$ , we obtain

$$\begin{aligned} x &\in (\{m\} \cup D(\beta) \cup (D(\gamma) + m)) \cap [m+n-1] \\ &= D(\beta\gamma) \quad (\text{by Proposition 5.6}). \end{aligned}$$

Combining this with  $x \in [m-1]$ , we obtain  $x \in D(\beta\gamma) \cap [m-1]$ .

Forget that we fixed  $x$ . We thus have shown that  $x \in D(\beta\gamma) \cap [m-1]$  for each  $x \in D(\beta)$ . In other words,

$$D(\beta) \subseteq D(\beta\gamma) \cap [m-1]. \quad (23)$$

On the other hand, let  $y \in D(\beta\gamma) \cap [m-1]$ . Thus,  $y \in D(\beta\gamma)$  and  $y \in [m-1]$ . From  $y \in [m-1] = \{1, 2, \dots, m-1\}$ , we obtain  $y \leq m-1 < m$ . Thus, we cannot have  $y \in \{m\}$  (because  $y \in \{m\}$  would entail  $y = m$ , which would contradict  $y < m$ ). Furthermore, we cannot have  $y \in D(\gamma) + m$  (because  $y \in D(\gamma) + m$  would entail that  $y \geq m$ <sup>7</sup>, which would contradict  $y < m$ ).

<sup>7</sup>Proof. Assume that  $y \in D(\gamma) + m$ . We must show that  $y \geq m$ .

We have  $y \in D(\gamma) + m = \{k+m \mid k \in D(\gamma)\}$  (by the definition of  $D(\gamma) + m$ ). In other words,  $y = k+m$  for some  $k \in D(\gamma)$ . Consider this  $k$ . From  $k \in D(\gamma) \subseteq [n-1] = \{1, 2, \dots, n-1\}$ , we obtain  $k \geq 1 > 0$ . Hence,  $y = \underbrace{k}_{>0} + m > m$ , thus  $y \geq m$ .

However,

$$\begin{aligned} y &\in D(\beta\gamma) \\ &= (\{m\} \cup D(\beta) \cup (D(\gamma) + m)) \cap [m + n - 1] \quad (\text{by Proposition 5.6}) \\ &\subseteq \{m\} \cup D(\beta) \cup (D(\gamma) + m). \end{aligned}$$

In other words, we have  $y \in \{m\}$  or  $y \in D(\beta)$  or  $y \in D(\gamma) + m$ . Hence, we must have  $y \in D(\beta)$  (since we cannot have  $y \in \{m\}$ , and we cannot have  $y \in D(\gamma) + m$ ).

Forget that we fixed  $y$ . We thus have shown that  $y \in D(\beta)$  for each  $y \in D(\beta\gamma) \cap [m - 1]$ . In other words,

$$D(\beta\gamma) \cap [m - 1] \subseteq D(\beta).$$

Combining this with (23), we obtain  $D(\beta) = D(\beta\gamma) \cap [m - 1]$ . This proves Proposition 5.7 (a).

(b) The definition of  $D(\gamma) + m$  yields

$$D(\gamma) + m = \{k + m \mid k \in D(\gamma)\}. \quad (24)$$

The definition of  $(D(\beta\gamma) \setminus [m]) - m$  yields

$$(D(\beta\gamma) \setminus [m]) - m = \{k - m \mid k \in D(\beta\gamma) \setminus [m]\}. \quad (25)$$

Let  $x \in D(\gamma)$ . We shall show that  $x \in (D(\beta\gamma) \setminus [m]) - m$ .

Indeed, we have  $x \in D(\gamma) \subseteq [n - 1] = \{1, 2, \dots, n - 1\}$ , so that

$$x + m \in \{m + 1, m + 2, \dots, m + n - 1\} \subseteq \{1, 2, \dots, m + n - 1\} = [m + n - 1].$$

Also, from  $x \in \{1, 2, \dots, n - 1\}$ , we obtain  $x \geq 1 > 0$ , and therefore  $\underbrace{x}_{>0} + m > m$ ,

so that  $x + m \notin [m]$ <sup>8</sup>.

Next, we recall that  $x \in D(\gamma)$ . Thus, the number  $x + m$  can be written in the form  $k + m$  for some  $k \in D(\gamma)$  (namely, for  $k = x$ ). In other words,  $x + m \in \{k + m \mid k \in D(\gamma)\}$ . In view of (24), we can rewrite this as  $x + m \in D(\gamma) + m$ . Hence,

$$x + m \in D(\gamma) + m \subseteq \{m\} \cup D(\beta) \cup (D(\gamma) + m).$$

Combining this with  $x + m \in [m + n - 1]$ , we obtain

$$\begin{aligned} x + m &\in (\{m\} \cup D(\beta) \cup (D(\gamma) + m)) \cap [m + n - 1] \\ &= D(\beta\gamma) \quad (\text{by Proposition 5.6}). \end{aligned}$$

Combining this with  $x + m \notin [m]$ , we obtain  $x + m \in D(\beta\gamma) \setminus [m]$ . We also have  $x = (x + m) - m$ . Therefore,  $x$  has the form  $k - m$  for some  $k \in D(\beta\gamma) \setminus [m]$

---

<sup>8</sup>*Proof.* If we had  $x + m \in [m]$ , then we would have  $x + m \leq m$  (since  $x + m \in [m] = \{1, 2, \dots, m\}$ ), but this would contradict  $x + m > m$ . Hence, we cannot have  $x + m \in [m]$ . In other words, we have  $x + m \notin [m]$ .

(namely, for  $k = x + m$ ), because  $x + m \in D(\beta\gamma) \setminus [m]$ . In other words,  $x \in \{k - m \mid k \in D(\beta\gamma) \setminus [m]\}$ . In view of (25), this rewrites as  $x \in (D(\beta\gamma) \setminus [m]) - m$ .

Forget that we fixed  $x$ . We thus have shown that  $x \in (D(\beta\gamma) \setminus [m]) - m$  for each  $x \in D(\gamma)$ . In other words,

$$D(\gamma) \subseteq (D(\beta\gamma) \setminus [m]) - m. \quad (26)$$

On the other hand, let  $y \in (D(\beta\gamma) \setminus [m]) - m$ . Thus,

$$y \in (D(\beta\gamma) \setminus [m]) - m = \{k - m \mid k \in D(\beta\gamma) \setminus [m]\}$$

(by (25)). In other words,  $y = k - m$  for some  $k \in D(\beta\gamma) \setminus [m]$ . Consider this  $k$ , and denote it by  $z$ . Thus,  $y = z - m$  and  $z \in D(\beta\gamma) \setminus [m]$ .

From  $z \in D(\beta\gamma) \setminus [m]$ , we obtain  $z \in D(\beta\gamma)$  and  $z \notin [m]$ . In particular,

$$\begin{aligned} z &\in D(\beta\gamma) \\ &= (\{m\} \cup D(\beta) \cup (D(\gamma) + m)) \cap [m + n - 1] \quad (\text{by Proposition 5.6}) \\ &\subseteq [m + n - 1] = \{1, 2, \dots, m + n - 1\}. \end{aligned}$$

Combining this with  $z \notin [m] = \{1, 2, \dots, m\}$ , we obtain

$$z \in \{1, 2, \dots, m + n - 1\} \setminus \{1, 2, \dots, m\} = \{m + 1, m + 2, \dots, m + n - 1\}.$$

Hence,  $z \geq m + 1 > m$ .

Furthermore,

$$\begin{aligned} z &\in (\{m\} \cup D(\beta) \cup (D(\gamma) + m)) \cap [m + n - 1] \\ &\subseteq \{m\} \cup D(\beta) \cup (D(\gamma) + m). \end{aligned}$$

In other words, we have  $z \in \{m\}$  or  $z \in D(\beta)$  or  $z \in D(\gamma) + m$ . However, we cannot have  $z \in \{m\}$ <sup>9</sup>, and we also cannot have  $z \in D(\beta)$ <sup>10</sup>. Hence, we must have  $z \in D(\gamma) + m$  (since we have  $z \in \{m\}$  or  $z \in D(\beta)$  or  $z \in D(\gamma) + m$ ). In view of (24), this rewrites as

$$z \in \{k + m \mid k \in D(\gamma)\}.$$

In other words,  $z = k + m$  for some  $k \in D(\gamma)$ . Consider this  $k$ . We have  $y = \underbrace{z}_{=k+m} - m = k + m - m = k \in D(\gamma)$ .

Forget that we fixed  $y$ . We thus have shown that  $y \in D(\gamma)$  for each  $y \in (D(\beta\gamma) \setminus [m]) - m$ . In other words,

$$(D(\beta\gamma) \setminus [m]) - m \subseteq D(\gamma).$$

Combining this with (26), we obtain  $(D(\beta\gamma) \setminus [m]) - m = D(\gamma)$ . This proves Proposition 5.7 (b).  $\square$

<sup>9</sup>*Proof.* Assume the contrary. Thus,  $z \in \{m\}$ . Hence,  $z = m$ , which contradicts  $z > m$ . This contradiction shows that our assumption was wrong. Thus, we cannot have  $z \in \{m\}$ .

<sup>10</sup>*Proof.* Assume the contrary. Thus,  $z \in D(\beta) \subseteq [m - 1] = \{1, 2, \dots, m - 1\}$ . Hence,  $z \leq m - 1 < m$ , which contradicts  $z > m$ . This contradiction shows that our assumption was wrong. Thus, we cannot have  $z \in D(\beta)$ .

## 5.4. Further lemmas

The next few propositions and lemmas will be used in a later proof.

**Proposition 5.8.** Let  $\beta, \gamma, \beta'$  and  $\gamma'$  be four compositions such that  $|\beta'| = |\beta|$  and  $D(\beta') \subseteq D(\beta)$  and  $|\gamma'| = |\gamma|$  and  $D(\gamma') \subseteq D(\gamma)$ . Then,  $D(\beta'\gamma') \subseteq D(\beta\gamma)$ .

*Proof of Proposition 5.8.* Let  $m = |\beta|$  and  $n = |\gamma|$ . Thus,  $|\beta'| = |\beta| = m$  and  $|\gamma'| = |\gamma| = n$ .

It is easy to see that if  $K$  and  $L$  are two sets of integers satisfying  $K \subseteq L$ , and if  $k$  is any integer, then  $K + k \subseteq L + k$ . Applying this to  $K = D(\gamma')$  and  $L = D(\gamma)$  and  $k = m$ , we obtain  $D(\gamma') + m \subseteq D(\gamma) + m$  (since  $D(\gamma') \subseteq D(\gamma)$ ).

Now, Proposition 5.6 yields

$$D(\beta\gamma) = (\{m\} \cup D(\beta) \cup (D(\gamma) + m)) \cap [m + n - 1]. \quad (27)$$

Also, we have  $m = |\beta'|$  (since  $|\beta'| = m$ ) and  $n = |\gamma'|$  (since  $|\gamma'| = n$ ). Hence, Proposition 5.6 (applied to  $\beta'$  and  $\gamma'$  instead of  $\beta$  and  $\gamma$ ) yields

$$\begin{aligned} D(\beta'\gamma') &= \left( \{m\} \cup \underbrace{D(\beta')}_{\subseteq D(\beta)} \cup \underbrace{(D(\gamma') + m)}_{\subseteq D(\gamma) + m} \right) \cap [m + n - 1] \\ &\subseteq (\{m\} \cup D(\beta) \cup (D(\gamma) + m)) \cap [m + n - 1] = D(\beta\gamma) \end{aligned}$$

(by (27)). This proves Proposition 5.8.  $\square$

**Proposition 5.9.** Let  $\alpha \in \text{Comp}$  be any composition, and let  $m \in \mathbb{N}$ . Then, there exists at most one pair  $(\beta, \gamma)$  of compositions such that  $|\beta| = m$  and  $\beta\gamma = \alpha$ .

*Proof of Proposition 5.9.* Let  $(\beta', \gamma')$  and  $(\beta'', \gamma'')$  be two pairs  $(\beta, \gamma)$  of compositions such that  $|\beta| = m$  and  $\beta\gamma = \alpha$ . Thus,  $(\beta', \gamma')$  and  $(\beta'', \gamma'')$  are two pairs of compositions and have the property that  $|\beta'| = m$  and  $\beta'\gamma' = \alpha$  and  $|\beta''| = m$  and  $\beta''\gamma'' = \alpha$ . Thus,  $\alpha = \beta''\gamma''$ .

We have  $m = |\beta'|$  (since  $|\beta'| = m$ ). Thus, Proposition 5.7 (a) (applied to  $\beta'$  and  $\gamma'$  instead of  $\beta$  and  $\gamma$ ) yields

$$D(\beta') = D\left(\underbrace{\beta'\gamma'}_{=\alpha}\right) \cap [m - 1] = D(\alpha) \cap [m - 1].$$

The same argument (applied to  $\beta''$  and  $\gamma''$  instead of  $\beta'$  and  $\gamma'$ ) yields

$$D(\beta'') = D(\alpha) \cap [m - 1].$$

Comparing these two equalities, we find  $D(\beta') = D(\beta'')$ .

Now,  $\beta'$  is a composition having size  $|\beta'| = m$ . In other words,  $\beta'$  is a composition of  $m$ . In other words,  $\beta' \in \text{Comp}_m$ . Similarly,  $\beta'' \in \text{Comp}_m$ .

Recall that the map  $D : \text{Comp}_n \rightarrow \mathcal{P}([n-1])$  is a bijection. Similarly, the map  $D : \text{Comp}_m \rightarrow \mathcal{P}([m-1])$  is a bijection. Hence, this map  $D$  is bijective, thus injective. In other words, if  $\varphi, \psi \in \text{Comp}_m$  satisfy  $D(\varphi) = D(\psi)$ , then  $\varphi = \psi$ . Applying this to  $\varphi = \beta'$  and  $\psi = \beta''$ , we obtain  $\beta' = \beta''$  (since  $\beta' \in \text{Comp}_m$  and  $\beta'' \in \text{Comp}_m$  and  $D(\beta') = D(\beta'')$ ).

Furthermore, Proposition 5.7 **(b)** (applied to  $\beta'$  and  $\gamma'$  instead of  $\beta$  and  $\gamma$ ) yields

$$D(\gamma') = \left( D \left( \underbrace{\beta' \gamma'}_{=\alpha} \right) \setminus [m] \right) - m = (D(\alpha) \setminus [m]) - m.$$

The same argument (applied to  $\beta''$  and  $\gamma''$  instead of  $\beta'$  and  $\gamma'$ ) yields

$$D(\gamma'') = (D(\alpha) \setminus [m]) - m.$$

Comparing these two equalities, we find  $D(\gamma') = D(\gamma'')$ .

Set  $n = |\gamma'|$ . Then, from  $\beta' \gamma' = \alpha$ , we obtain  $\alpha = \beta' \gamma'$ . Thus,

$$\begin{aligned} |\alpha| &= |\beta' \gamma'| = \underbrace{|\beta'|}_{=m} + \underbrace{|\gamma'|}_{=n} && \left( \begin{array}{l} \text{by Proposition 5.2 (b),} \\ \text{applied to } \beta = \beta' \text{ and } \gamma = \gamma' \end{array} \right) \\ &= m + n. \end{aligned}$$

Hence,

$$\begin{aligned} m + n &= |\alpha| = |\beta'' \gamma''| && (\text{since } \alpha = \beta'' \gamma'') \\ &= \underbrace{|\beta''|}_{=m} + |\gamma''| && \left( \begin{array}{l} \text{by Proposition 5.2 (b),} \\ \text{applied to } \beta = \beta'' \text{ and } \gamma = \gamma'' \end{array} \right) \\ &= m + |\gamma''|. \end{aligned}$$

Subtracting  $m$  from this equality, we obtain  $n = |\gamma''|$ .

Now,  $\gamma'$  is a composition having size  $|\gamma'| = n$  (since  $n = |\gamma'|$ ). In other words,  $\gamma'$  is a composition of  $n$ . In other words,  $\gamma' \in \text{Comp}_n$ . Similarly,  $\gamma'' \in \text{Comp}_n$  (since  $n = |\gamma''|$ ).

Recall that the map  $D : \text{Comp}_n \rightarrow \mathcal{P}([n-1])$  is a bijection. Hence, this map  $D$  is bijective, thus injective. In other words, if  $\varphi, \psi \in \text{Comp}_n$  satisfy  $D(\varphi) = D(\psi)$ , then  $\varphi = \psi$ . Applying this to  $\varphi = \gamma'$  and  $\psi = \gamma''$ , we obtain  $\gamma' = \gamma''$  (since  $\gamma' \in \text{Comp}_n$  and  $\gamma'' \in \text{Comp}_n$  and  $D(\gamma') = D(\gamma'')$ ).

$$\text{Now, } \left( \underbrace{\beta'}_{=\beta''}, \underbrace{\gamma'}_{=\gamma''} \right) = (\beta'', \gamma'').$$

Forget that we fixed  $(\beta', \gamma')$  and  $(\beta'', \gamma'')$ . We thus have shown that if  $(\beta', \gamma')$  and  $(\beta'', \gamma'')$  are two pairs  $(\beta, \gamma)$  of compositions such that  $|\beta| = m$  and  $\beta\gamma = \alpha$ , then  $(\beta', \gamma') = (\beta'', \gamma'')$ . In other words, there exists at most one pair  $(\beta, \gamma)$  of compositions such that  $|\beta| = m$  and  $\beta\gamma = \alpha$ . This proves Proposition 5.9.  $\square$

Next, we shall show a nearly trivial lemma:

**Lemma 5.10.** Let  $m \in \mathbb{N}$ . Let  $K$  be a subset of  $\{1, 2, 3, \dots\}$ . Then,

$$(K \cap [m-1]) \cup (K \setminus [m]) = K \setminus \{m\}.$$

*Proof of Lemma 5.10.* Any element  $k \in K$  is an element of  $\{1, 2, 3, \dots\}$  (since  $K$  is a subset of  $\{1, 2, 3, \dots\}$ ) and therefore is a positive integer. Hence, for any element  $k \in K$ , we have the following chain of logical equivalences:

$$\begin{aligned} (k \in [m-1]) &\iff (k \leq m-1) && \text{(since } k \text{ is a positive integer)} \\ &\iff (k < m) && \text{(since } k \text{ and } m \text{ are integers).} \end{aligned}$$

Thus,

$$\{k \in K \mid k \in [m-1]\} = \{k \in K \mid k < m\}.$$

Recall again that any element  $k \in K$  is a positive integer. Hence, for any element  $k \in K$ , we have the following chain of logical equivalences:

$$\begin{aligned} (k \notin [m]) &\iff (\text{we don't have } k \in [m]) \\ &\iff (\text{we don't have } k \leq m) && \left( \begin{array}{l} \text{since } k \text{ is a positive integer,} \\ \text{and thus the statement " } k \in [m] \text{ " } \\ \text{is equivalent to " } k \leq m \text{ " } \end{array} \right) \\ &\iff (k > m). \end{aligned}$$

Hence,

$$\{k \in K \mid k \notin [m]\} = \{k \in K \mid k > m\}.$$

Now,

$$\begin{aligned} &\underbrace{(K \cap [m-1])}_{=\{k \in K \mid k \in [m-1]\}} \cup \underbrace{(K \setminus [m])}_{=\{k \in K \mid k \notin [m]\}} \\ &= \underbrace{\{k \in K \mid k \in [m-1]\}}_{=\{k \in K \mid k < m\}} \cup \underbrace{\{k \in K \mid k \notin [m]\}}_{=\{k \in K \mid k > m\}} \\ &= \{k \in K \mid k < m\} \cup \{k \in K \mid k > m\} \\ &= \{k \in K \mid k < m \text{ or } k > m\} \\ &= \{k \in K \mid k \neq m\} && \left( \begin{array}{l} \text{since the statement " } k < m \text{ or } k > m \text{ " } \\ \text{is equivalent to " } k \neq m \text{ " } \end{array} \right) \\ &= K \setminus \{m\}. \end{aligned}$$

This proves Lemma 5.10. □

Our next proposition characterizes the concatenation  $\varphi\psi$  of two compositions  $\varphi$  and  $\psi$  in terms of how its partial sum set  $D(\alpha)$  relates to  $D(\varphi)$  and  $D(\psi)$ :

**Proposition 5.11.** Let  $n \in \mathbb{N}$  and  $m \in \mathbb{N}$ . Let  $\alpha \in \text{Comp}_{m+n}$  be any composition of  $m+n$  such that  $m \in D(\alpha) \cup \{0, m+n\}$ .

Let  $\varphi \in \text{Comp}_m$  be a composition that satisfies  $D(\varphi) = D(\alpha) \cap [m-1]$ .

Let  $\psi \in \text{Comp}_n$  be a composition that satisfies  $D(\psi) = (D(\alpha) \setminus [m]) - m$ .

Then,  $\varphi\psi = \alpha$ .

*Proof of Proposition 5.11.* We have  $\varphi \in \text{Comp}_m$ . In other words,  $\varphi$  is a composition of  $m$ . In other words,  $\varphi$  is a composition having size  $m$ . In other words,  $\varphi \in \text{Comp}$  and  $|\varphi| = m$ . Similarly, from  $\psi \in \text{Comp}_n$ , we obtain  $\psi \in \text{Comp}$  and  $|\psi| = n$ .

Now, Proposition 5.2 (b) (applied to  $\beta = \varphi$  and  $\gamma = \psi$ ) yields  $|\varphi\psi| = \underbrace{|\varphi|}_{=m} + \underbrace{|\psi|}_{=n} =$

$m+n$ . Thus,  $\varphi\psi$  is a composition having size  $|\varphi\psi| = m+n$ . In other words,  $\varphi\psi$  is a composition of  $m+n$ . In other words,  $\varphi\psi \in \text{Comp}_{m+n}$ .

Recall that the map  $D : \text{Comp}_{m+n} \rightarrow \mathcal{P}([m+n-1])$  is a bijection. Hence, this map  $D$  is bijective, thus injective. Furthermore, from  $\alpha \in \text{Comp}_{m+n}$ , we obtain  $D(\alpha) \in \mathcal{P}([m+n-1])$  (since  $D$  is a map from  $\text{Comp}_{m+n}$  to  $\mathcal{P}([m+n-1])$ ). In other words,  $D(\alpha) \subseteq [m+n-1]$ . Hence,

$$D(\alpha) \subseteq [m+n-1] \subseteq \{1, 2, 3, \dots\}.$$

In other words,  $D(\alpha)$  is a subset of  $\{1, 2, 3, \dots\}$ . Hence, Lemma 5.10 (applied to  $K = D(\alpha)$ ) yields

$$(D(\alpha) \cap [m-1]) \cup (D(\alpha) \setminus [m]) = D(\alpha) \setminus \{m\}. \quad (28)$$

If  $K$  is any set of integers, then  $(K - m) + m = K$  (indeed, this follows easily from Definition 5.4). Applying this to  $K = D(\alpha) \setminus [m]$ , we obtain

$$((D(\alpha) \setminus [m]) - m) + m = D(\alpha) \setminus [m].$$

In view of  $D(\psi) = (D(\alpha) \setminus [m]) - m$ , we can rewrite this as

$$D(\psi) + m = D(\alpha) \setminus [m]. \quad (29)$$



Proposition 5.6 (applied to  $\beta = \varphi$  and  $\gamma = \psi$ ) yields

$$\begin{aligned}
 D(\varphi\psi) &= \left( \{m\} \cup \underbrace{D(\varphi)}_{=D(\alpha)\cap[m-1]} \cup \underbrace{(D(\psi)+m)}_{\substack{=D(\alpha)\setminus[m] \\ \text{(by (29))}}} \right) \cap [m+n-1] \\
 &= \left( \{m\} \cup \underbrace{(D(\alpha)\cap[m-1]) \cup (D(\alpha)\setminus[m])}_{\substack{=D(\alpha)\setminus\{m\} \\ \text{(by (28))}}} \right) \cap [m+n-1] \\
 &= \underbrace{(\{m\} \cup (D(\alpha)\setminus\{m\}))}_{\substack{=\{m\}\cup D(\alpha) \\ \text{(since } (X\cup(Y\setminus X))=X\cup Y \\ \text{for any two sets } X \text{ and } Y)}} \cap [m+n-1] \\
 &= (\{m\} \cup D(\alpha)) \cap [m+n-1]. \tag{30}
 \end{aligned}$$

Now, we recall that  $m \in D(\alpha) \cup \{0, m+n\}$  (by assumption). Hence,  $\{m\} \subseteq D(\alpha) \cup \{0, m+n\}$ . Thus,

$$\begin{aligned}
 \underbrace{\{m\}}_{\subseteq D(\alpha)\cup\{0,m+n\}} \cup D(\alpha) &\subseteq (D(\alpha) \cup \{0, m+n\}) \cup D(\alpha) \\
 &= \underbrace{D(\alpha) \cup D(\alpha)}_{=D(\alpha)} \cup \{0, m+n\} \\
 &= D(\alpha) \cup \{0, m+n\}.
 \end{aligned}$$

Hence,

$$\begin{aligned}
 &\underbrace{(\{m\} \cup D(\alpha))}_{\subseteq D(\alpha)\cup\{0,m+n\}} \cap [m+n-1] \\
 &\subseteq (D(\alpha) \cup \{0, m+n\}) \cap [m+n-1] \\
 &= (D(\alpha) \cap [m+n-1]) \cup \underbrace{(\{0, m+n\} \cap [m+n-1])}_{\substack{=\emptyset \\ \text{(since neither 0 nor } m+n \text{ belongs} \\ \text{to the set } [m+n-1])}} \\
 &\quad \left( \begin{array}{c} \text{since } (X \cup Y) \cap Z = (X \cap Z) \cup (Y \cap Z) \\ \text{for any three sets } X, Y \text{ and } Z \end{array} \right) \\
 &= (D(\alpha) \cap [m+n-1]) \cup \emptyset = D(\alpha) \cap [m+n-1] \\
 &= D(\alpha) \quad (\text{since } D(\alpha) \subseteq [m+n-1]).
 \end{aligned}$$


---

Combining this inclusion with

$$\begin{aligned} D(\alpha) &= \underbrace{D(\alpha)}_{\subseteq (\{m\} \cup D(\alpha))} \cap [m+n-1] \quad (\text{since } D(\alpha) \subseteq [m+n-1]) \\ &\subseteq (\{m\} \cup D(\alpha)) \cap [m+n-1], \end{aligned}$$

we obtain

$$(\{m\} \cup D(\alpha)) \cap [m+n-1] = D(\alpha).$$

Hence, we can rewrite (30) as  $D(\varphi\psi) = D(\alpha)$ .

Now, recall that the map  $D : \text{Comp}_{m+n} \rightarrow \mathcal{P}([m+n-1])$  is injective. Hence, if  $\zeta$  and  $\eta$  are two elements of  $\text{Comp}_{m+n}$  satisfying  $D(\zeta) = D(\eta)$ , then  $\zeta = \eta$ . Applying this to  $\zeta = \varphi\psi$  and  $\eta = \alpha$ , we obtain  $\varphi\psi = \alpha$  (since  $\varphi\psi \in \text{Comp}_{m+n}$  and  $\alpha \in \text{Comp}_{m+n}$  and  $D(\varphi\psi) = D(\alpha)$ ). This proves Proposition 5.11.  $\square$

## 5.5. Concatenation and coarsenings

We shall next study the interaction between concatenation and coarsenings. First, we define coarsenings:

**Definition 5.12.** If  $\gamma$  is a composition, then  $C(\gamma)$  shall denote the set of all compositions  $\beta \in \text{Comp}_{|\gamma|}$  satisfying  $D(\beta) \subseteq D(\gamma)$ .

The compositions belonging to  $C(\gamma)$  are often called the *coarsenings* of  $\gamma$ .

**Example 5.13.** Let  $\gamma$  be the composition  $(4, 1, 2)$ . Then, the set  $C(\gamma)$  consists of the compositions  $\beta \in \text{Comp}_7$  satisfying  $D(\beta) \subseteq D(\gamma) = \{4, 5\}$ . Thus,

$$C(\gamma) = \{(7), (5, 2), (4, 3), (4, 1, 2)\}.$$

So the coarsenings of  $\gamma$  are the four compositions  $(7)$ ,  $(5, 2)$ ,  $(4, 3)$  and  $(4, 1, 2)$ .

An equivalent definition of the coarsenings of a composition  $\gamma$  can be informally given as follows: If  $\gamma$  is a composition, then a *coarsening* of  $\gamma$  means a composition obtained by “combining” some groups of consecutive entries of  $\gamma$  (that is, replacing them by their sums). For instance, one of the many coarsenings of a composition  $(\alpha_1, \alpha_2, \alpha_3, \alpha_4, \alpha_5, \alpha_6, \alpha_7)$  is  $(\alpha_1 + \alpha_2, \alpha_3, \alpha_4 + \alpha_5 + \alpha_6, \alpha_7)$ . We shall not formalize this equivalent definition, as we will not use it.

The following lemma is a trivial consequence of the definition of a coarsening, restated for convenience:

**Lemma 5.14.** Let  $\gamma$  be a composition.

- (a) If  $\nu \in C(\gamma)$ , then  $\nu \in \text{Comp}$  and  $|\nu| = |\gamma|$  and  $D(\nu) \subseteq D(\gamma)$ .
- (b) If  $\nu \in \text{Comp}$  is a composition that satisfies  $|\nu| = |\gamma|$  and  $D(\nu) \subseteq D(\gamma)$ , then  $\nu \in C(\gamma)$ .

*Proof.* **(a)** Assume that  $\nu \in C(\gamma)$ . According to the definition of  $C(\gamma)$ , this means that  $\nu$  is a composition  $\beta \in \text{Comp}_{|\gamma|}$  satisfying  $D(\beta) \subseteq D(\gamma)$ . In other words,  $\nu \in \text{Comp}_{|\gamma|}$  and  $D(\nu) \subseteq D(\gamma)$ . From  $\nu \in \text{Comp}_{|\gamma|}$ , we obtain  $\nu \in \text{Comp}$  and  $|\nu| = |\gamma|$ . Thus, we have  $\nu \in \text{Comp}$  and  $|\nu| = |\gamma|$  and  $D(\nu) \subseteq D(\gamma)$ . This proves Lemma 5.14 **(a)**.

**(b)** Assume that  $\nu \in \text{Comp}$  is a composition that satisfies  $|\nu| = |\gamma|$  and  $D(\nu) \subseteq D(\gamma)$ . From  $\nu \in \text{Comp}$  and  $|\nu| = |\gamma|$ , we obtain  $\nu \in \text{Comp}_{|\gamma|}$ . Thus,  $\nu$  is a composition  $\beta \in \text{Comp}_{|\gamma|}$  satisfying  $D(\beta) \subseteq D(\gamma)$  (since  $D(\nu) \subseteq D(\gamma)$ ). In other words,  $\nu \in C(\gamma)$  (by the definition of  $C(\gamma)$ ). This proves Lemma 5.14 **(b)**.  $\square$

We can now restate Proposition 5.8 in terms of coarsenings:

**Proposition 5.15.** Let  $\beta$  and  $\gamma$  be two compositions. Let  $\mu \in C(\beta)$  and  $\nu \in C(\gamma)$ . Then,  $\mu\nu \in C(\beta\gamma)$ .

*Proof of Proposition 5.15.* We have  $\nu \in C(\gamma)$ . Thus, Lemma 5.14 **(a)** yields that  $\nu \in \text{Comp}$  and  $|\nu| = |\gamma|$  and  $D(\nu) \subseteq D(\gamma)$ . The same argument (applied to  $\mu$  and  $\beta$  instead of  $\nu$  and  $\gamma$ ) shows that  $\mu \in \text{Comp}$  and  $|\mu| = |\beta|$  and  $D(\mu) \subseteq D(\beta)$ . Hence, Proposition 5.8 (applied to  $\beta' = \mu$  and  $\gamma' = \nu$ ) yields  $D(\mu\nu) \subseteq D(\beta\gamma)$ .

However, Proposition 5.2 **(b)** yields  $|\beta\gamma| = |\beta| + |\gamma|$ .

Furthermore, Proposition 5.2 **(b)** (applied to  $\mu$  and  $\nu$  instead of  $\beta$  and  $\gamma$ ) yields

$$|\mu\nu| = \underbrace{|\mu|}_{=|\beta|} + \underbrace{|\nu|}_{=|\gamma|} = |\beta| + |\gamma| = |\beta\gamma| \quad (\text{since } |\beta\gamma| = |\beta| + |\gamma|).$$

Thus, we now know that  $\mu\nu \in \text{Comp}$  and  $|\mu\nu| = |\beta\gamma|$  and  $D(\mu\nu) \subseteq D(\beta\gamma)$ . Hence, Lemma 5.14 **(b)** (applied to  $\beta\gamma$  and  $\mu\nu$  instead of  $\gamma$  and  $\nu$ ) yields that  $\mu\nu \in C(\beta\gamma)$ . This proves Proposition 5.15.  $\square$

The following proposition is a sort of converse to Proposition 5.15:

**Proposition 5.16.** Let  $\alpha$  be a composition. Let  $\mu$  and  $\nu$  be two compositions satisfying  $\mu\nu \in C(\alpha)$ . Then, there exists a unique pair  $(\beta, \gamma) \in \text{Comp} \times \text{Comp}$  of compositions satisfying  $\beta\gamma = \alpha$  and  $\mu \in C(\beta)$  and  $\nu \in C(\gamma)$ .

*Proof of Proposition 5.16.* Let  $m = |\mu|$  and  $n = |\nu|$ . Then,  $\mu \in \text{Comp}_m$  (since  $\mu$  is a composition that satisfies  $|\mu| = m$ ) and  $\nu \in \text{Comp}_n$  (since  $\nu$  is a composition that satisfies  $|\nu| = n$ ). Also, from  $\mu\nu \in C(\alpha)$ , we conclude (by the definition of  $C(\alpha)$ ) that  $\mu\nu \in \text{Comp}_{|\alpha|}$  and  $D(\mu\nu) \subseteq D(\alpha)$ . Now, from  $\mu\nu \in \text{Comp}_{|\alpha|}$ , we obtain  $|\mu\nu| = |\alpha|$ . Thus,  $|\alpha| = |\mu\nu|$ .

On the other hand, Proposition 5.2 **(b)** (applied to  $\beta = \mu$  and  $\gamma = \nu$ ) yields

$$|\mu\nu| = \underbrace{|\mu|}_{=m} + \underbrace{|\nu|}_{=n} = m + n.$$

Hence,  $|\alpha| = |\mu\nu| = m + n$ , so that  $\alpha \in \text{Comp}_{m+n}$ . Thus,  $D(\alpha) \in \mathcal{P}([m+n-1])$  (since  $D : \text{Comp}_{m+n} \rightarrow \mathcal{P}([m+n-1])$  is a bijection). In other words,  $D(\alpha) \subseteq [m+n-1]$ .

It is furthermore easy to see that

$$m \in D(\alpha) \cup \{0, m+n\}$$

<sup>11</sup>.

We have  $D(\alpha) \cap [m-1] \subseteq [m-1]$ , so that  $D(\alpha) \cap [m-1] \in \mathcal{P}([m-1])$ .

Furthermore, it is easy to see that  $(D(\alpha) \setminus [m]) - m \in \mathcal{P}([n-1])$  <sup>12</sup>.

Recall that the map  $D : \text{Comp}_m \rightarrow \mathcal{P}([m-1])$  is a bijection. Hence, it is bijective, thus surjective. Therefore, there exists some composition  $\varphi \in \text{Comp}_m$  that satisfies

$$D(\varphi) = D(\alpha) \cap [m-1] \quad (32)$$

<sup>11</sup>Proof. We are in one of the following three cases:

Case 1: We have  $m = 0$ .

Case 2: We have  $n = 0$ .

Case 3: We have neither  $m = 0$  nor  $n = 0$ .

Let us first consider Case 1. In this case, we have  $m = 0$ . Hence,  $m = 0 \in \{0, m+n\} \subseteq D(\alpha) \cup \{0, m+n\}$ . Thus,  $m \in D(\alpha) \cup \{0, m+n\}$  is proved in Case 1.

Let us next consider Case 2. In this case, we have  $n = 0$ . Hence,  $m + \underbrace{n}_{=0} = m$ , so that

$m = m + n \in \{0, m+n\} \subseteq D(\alpha) \cup \{0, m+n\}$ . Thus,  $m \in D(\alpha) \cup \{0, m+n\}$  is proved in Case 2.

Now, let us consider Case 3. In this case, we have neither  $m = 0$  nor  $n = 0$ . Hence,  $m \neq 0$  and  $n \neq 0$ . Therefore,  $\mu \neq \emptyset$  (since  $|\mu| = m \neq 0 = |\emptyset|$ ) and  $\nu \neq \emptyset$  (since  $|\nu| = n \neq 0 = |\emptyset|$ ). Hence, Proposition 5.5 (applied to  $\mu$  and  $\nu$  instead of  $\beta$  and  $\gamma$ ) yields

$$D(\mu\nu) = \{m\} \cup D(\mu) \cup (D(\nu) + m). \quad (31)$$

Now,

$$\begin{aligned} m \in \{m\} &\subseteq \{m\} \cup D(\mu) \cup (D(\nu) + m) \\ &= D(\mu\nu) \quad (\text{by (31)}) \\ &\subseteq D(\alpha) \subseteq D(\alpha) \cup \{0, m+n\}. \end{aligned}$$

Thus,  $m \in D(\alpha) \cup \{0, m+n\}$  is proved in Case 3.

Hence, we have proved  $m \in D(\alpha) \cup \{0, m+n\}$  in all three Cases 1, 2 and 3. Thus,  $m \in D(\alpha) \cup \{0, m+n\}$  always holds.

<sup>12</sup>Proof. Let  $g \in (D(\alpha) \setminus [m]) - m$ . We shall show that  $g \in [n-1]$ .

Indeed,

$$g \in (D(\alpha) \setminus [m]) - m = \{k - m \mid k \in D(\alpha) \setminus [m]\}$$

(by the definition of  $(D(\alpha) \setminus [m]) - m$ ). In other words,  $g = k - m$  for some  $k \in D(\alpha) \setminus [m]$ . Consider this  $k$ .

We have  $k \in D(\alpha) \setminus [m]$ , so that  $k \in D(\alpha)$  and  $k \notin [m]$ . From  $k \in D(\alpha) \subseteq [m+n-1]$ , we obtain  $1 \leq k \leq m+n-1$ . If we had  $k \leq m$ , then we would have  $k \in [m]$  (since  $1 \leq k \leq m$ ), which would contradict  $k \notin [m]$ . Thus, we cannot have  $k \leq m$ . Hence, we must have  $k > m$ . Thus,  $k \geq m+1$  (since  $k$  and  $m$  are integers), so that  $k - m \geq 1$ . Furthermore, from  $k \leq m+n-1$ , we obtain  $k - m \leq n-1$ . Combining  $k - m \geq 1$  with  $k - m \leq n-1$ , we find  $k - m \in \{1, 2, \dots, n-1\} = [n-1]$ . Thus,  $g = k - m \in [n-1]$ .

Forget now that we fixed  $g$ . We thus have shown that  $g \in [n-1]$  for each  $g \in (D(\alpha) \setminus [m]) - m$ . In other words,  $(D(\alpha) \setminus [m]) - m \subseteq [n-1]$ . In other words,  $(D(\alpha) \setminus [m]) - m \in \mathcal{P}([n-1])$ .

(since  $D(\alpha) \cap [m-1] \in \mathcal{P}([m-1])$ ). Consider this  $\varphi$ .

Recall that the map  $D : \text{Comp}_n \rightarrow \mathcal{P}([n-1])$  is a bijection. Hence, it is bijective, thus surjective. Therefore, there exists some composition  $\psi \in \text{Comp}_n$  that satisfies

$$D(\psi) = (D(\alpha) \setminus [m]) - m \quad (33)$$

(since  $(D(\alpha) \setminus [m]) - m \in \mathcal{P}([n-1])$ ). Consider this  $\psi$ .

Proposition 5.11 yields that

$$\varphi\psi = \alpha.$$

Also,  $\varphi \in \text{Comp}_m \subseteq \text{Comp}$  and  $|\varphi| = m$  (since  $\varphi \in \text{Comp}_m$ ). Furthermore,  $\psi \in \text{Comp}_n \subseteq \text{Comp}$  and  $|\psi| = n$  (since  $\psi \in \text{Comp}_n$ ). From  $\varphi \in \text{Comp}$  and  $\psi \in \text{Comp}$ , we obtain  $(\varphi, \psi) \in \text{Comp} \times \text{Comp}$ .

Proposition 5.7 (a) (applied to  $\beta = \mu$  and  $\gamma = \nu$ ) yields

$$D(\mu) = \underbrace{D(\mu\nu) \cap [m-1]}_{\subseteq D(\alpha)} \subseteq D(\alpha) \cap [m-1] = D(\varphi)$$

(by (32)). Also, we have  $|\mu| = m = |\varphi|$  (since  $|\varphi| = m$ ), so that  $\mu \in \text{Comp}_{|\varphi|}$ . Thus,  $\mu$  is a composition  $\beta \in \text{Comp}_{|\varphi|}$  satisfying  $D(\beta) \subseteq D(\varphi)$  (since we have shown that  $D(\mu) \subseteq D(\varphi)$ ). In other words,  $\mu \in C(\varphi)$  (by the definition of  $C(\varphi)$ ).

Proposition 5.7 (b) (applied to  $\beta = \mu$  and  $\gamma = \nu$ ) yields

$$D(\nu) = (D(\mu\nu) \setminus [m]) - m. \quad (34)$$

However,  $\underbrace{D(\mu\nu) \setminus [m]}_{\subseteq D(\alpha)} \subseteq D(\alpha) \setminus [m]$ . But it is easy to see that if  $k$  is any integer,

and if  $K$  and  $K'$  are two sets of integers satisfying  $K \subseteq K'$ , then  $K - k \subseteq K' - k$ . Applying this to  $k = m$  and  $K = D(\mu\nu) \setminus [m]$  and  $K' = D(\alpha) \setminus [m]$ , we conclude that  $(D(\mu\nu) \setminus [m]) - m \subseteq (D(\alpha) \setminus [m]) - m$  (since  $D(\mu\nu) \setminus [m] \subseteq D(\alpha) \setminus [m]$ ). In view of (34), we can rewrite this as

$$D(\nu) = (D(\alpha) \setminus [m]) - m = D(\psi)$$

(by (33)). Also, we have  $|\nu| = n = |\psi|$  (since  $|\psi| = n$ ), so that  $\nu \in \text{Comp}_{|\psi|}$ . Thus,  $\nu$  is a composition  $\beta \in \text{Comp}_{|\psi|}$  satisfying  $D(\beta) \subseteq D(\psi)$  (since we have shown that  $D(\nu) \subseteq D(\psi)$ ). In other words,  $\nu \in C(\psi)$  (by the definition of  $C(\psi)$ ).

We have now shown that  $(\varphi, \psi) \in \text{Comp} \times \text{Comp}$  is a pair of compositions satisfying  $\varphi\psi = \alpha$  and  $\mu \in C(\varphi)$  and  $\nu \in C(\psi)$ . Hence, there exists **at least** one pair  $(\beta, \gamma) \in \text{Comp} \times \text{Comp}$  of compositions satisfying  $\beta\gamma = \alpha$  and  $\mu \in C(\beta)$  and  $\nu \in C(\gamma)$  (namely, the pair  $(\varphi, \psi)$ ).

It remains to show that there exists **only** one such pair. So let us show this now.

Indeed, let  $(\beta', \gamma')$  and  $(\beta'', \gamma'')$  be two pairs  $(\beta, \gamma) \in \text{Comp} \times \text{Comp}$  of compositions satisfying  $\beta\gamma = \alpha$  and  $\mu \in C(\beta)$  and  $\nu \in C(\gamma)$ . We must prove that  $(\beta', \gamma') = (\beta'', \gamma'')$ .

We know that  $(\beta', \gamma')$  is a pair  $(\beta, \gamma) \in \text{Comp} \times \text{Comp}$  of compositions satisfying  $\beta\gamma = \alpha$  and  $\mu \in C(\beta)$  and  $\nu \in C(\gamma)$ . In other words,  $(\beta', \gamma') \in \text{Comp} \times \text{Comp}$  is a pair of compositions satisfying  $\beta'\gamma' = \alpha$  and  $\mu \in C(\beta')$  and  $\nu \in C(\gamma')$ . From  $\mu \in C(\beta')$ , we easily obtain  $|\beta'| = m$ <sup>13</sup>.

We have now shown that  $|\beta'| = m$  and  $\beta'\gamma' = \alpha$ . In other words,  $(\beta', \gamma')$  is a pair  $(\beta, \gamma)$  of compositions such that  $|\beta| = m$  and  $\beta\gamma = \alpha$ . The same argument (applied to  $(\beta'', \gamma'')$  instead of  $(\beta', \gamma')$ ) shows that  $(\beta'', \gamma'')$  is such a pair as well.

However, Proposition 5.9 shows that there exists at most one pair  $(\beta, \gamma)$  of compositions such that  $|\beta| = m$  and  $\beta\gamma = \alpha$ . Hence, any two such pairs  $(\beta, \gamma)$  must be equal. Since  $(\beta', \gamma')$  and  $(\beta'', \gamma'')$  are two such pairs (as we have shown in the previous paragraph), we thus can conclude that  $(\beta', \gamma')$  and  $(\beta'', \gamma'')$  must be equal. In other words,  $(\beta', \gamma') = (\beta'', \gamma'')$ .

Now, forget that we fixed  $(\beta', \gamma')$  and  $(\beta'', \gamma'')$ . We thus have shown that if  $(\beta', \gamma')$  and  $(\beta'', \gamma'')$  are two pairs  $(\beta, \gamma) \in \text{Comp} \times \text{Comp}$  of compositions satisfying  $\beta\gamma = \alpha$  and  $\mu \in C(\beta)$  and  $\nu \in C(\gamma)$ , then  $(\beta', \gamma') = (\beta'', \gamma'')$ . In other words, any two pairs  $(\beta, \gamma) \in \text{Comp} \times \text{Comp}$  of compositions satisfying  $\beta\gamma = \alpha$  and  $\mu \in C(\beta)$  and  $\nu \in C(\gamma)$  must be equal. In other words, there exists **at most one** such pair  $(\beta, \gamma)$ . Since we also know that there exists **at least one** such pair  $(\beta, \gamma)$  (because we have proved this further above), we thus conclude that there exists a **unique** such pair  $(\beta, \gamma)$ . This proves Proposition 5.16.  $\square$

We can combine Propositions 5.15 and 5.16 into a convenient package:

**Proposition 5.17.** Let  $(A, +, 0)$  be an abelian group. Let  $u_{\mu, \nu}$  be an element of  $A$  for each pair  $(\mu, \nu) \in \text{Comp} \times \text{Comp}$  of two compositions. Let  $\alpha \in \text{Comp}$ . Then,

$$\sum_{\substack{(\mu, \nu) \in \text{Comp} \times \text{Comp}; \\ \mu\nu \in C(\alpha)}} u_{\mu, \nu} = \sum_{\substack{(\beta, \gamma) \in \text{Comp} \times \text{Comp}; \\ \beta\gamma = \alpha}} \sum_{\mu \in C(\beta)} \sum_{\nu \in C(\gamma)} u_{\mu, \nu}.$$

<sup>13</sup>*Proof.* We have  $\mu \in C(\beta')$ . By the definition of  $C(\beta')$ , this means that  $\mu$  is a composition  $\beta \in \text{Comp}_{|\beta'|}$  satisfying  $D(\beta) \subseteq D(\beta')$ . In other words,  $\mu \in \text{Comp}_{|\beta'|}$  and  $D(\mu) \subseteq D(\beta')$ . Hence,  $\mu \in \text{Comp}_{|\beta'|}$ , so that  $|\mu| = |\beta'|$ . Thus,  $|\beta'| = |\mu| = m$ .

*Proof of Proposition 5.17.* We have

$$\begin{aligned}
& \sum_{\substack{(\beta, \gamma) \in \text{Comp} \times \text{Comp}; \\ \beta\gamma = \alpha}} \sum_{\substack{\mu \in C(\beta)}} \sum_{\substack{v \in C(\gamma)}} u_{\mu, v} \\
&= \sum_{\substack{\mu \in \text{Comp}; \\ \mu \in C(\beta)}} \sum_{\substack{v \in \text{Comp}; \\ v \in C(\gamma)}} u_{\mu, v} \quad (\text{since } C(\beta) \subseteq \text{Comp}) \quad (\text{since } C(\gamma) \subseteq \text{Comp}) \\
&= \sum_{\substack{(\beta, \gamma) \in \text{Comp} \times \text{Comp}; \\ \beta\gamma = \alpha}} \sum_{\substack{\mu \in \text{Comp}; \\ \mu \in C(\beta)}} \sum_{\substack{v \in \text{Comp}; \\ v \in C(\gamma)}} u_{\mu, v} \\
&= \sum_{\mu \in \text{Comp}} \sum_{v \in \text{Comp}} \sum_{\substack{(\beta, \gamma) \in \text{Comp} \times \text{Comp}; \\ \beta\gamma = \alpha; \\ \mu \in C(\beta); \\ v \in C(\gamma)}} u_{\mu, v} \\
&= \sum_{\mu \in \text{Comp}} \sum_{v \in \text{Comp}} \sum_{\substack{(\beta, \gamma) \in \text{Comp} \times \text{Comp}; \\ \beta\gamma = \alpha; \\ \mu \in C(\beta); \\ v \in C(\gamma)}} u_{\mu, v} \\
&= \sum_{(\mu, v) \in \text{Comp} \times \text{Comp}} \sum_{\substack{(\beta, \gamma) \in \text{Comp} \times \text{Comp}; \\ \beta\gamma = \alpha; \\ \mu \in C(\beta); \\ v \in C(\gamma)}} u_{\mu, v}. \tag{35}
\end{aligned}$$

Now, we claim the following:

*Claim 1:* Let  $(\mu, v) \in \text{Comp} \times \text{Comp}$  be such that  $\mu v \in C(\alpha)$ . Then,

$$\sum_{\substack{(\beta, \gamma) \in \text{Comp} \times \text{Comp}; \\ \beta\gamma = \alpha; \\ \mu \in C(\beta); \\ v \in C(\gamma)}} u_{\mu, v} = u_{\mu, v}.$$

[*Proof of Claim 1:* Proposition 5.16 shows that there exists a unique pair  $(\beta, \gamma) \in \text{Comp} \times \text{Comp}$  of compositions satisfying  $\beta\gamma = \alpha$  and  $\mu \in C(\beta)$  and  $v \in C(\gamma)$ . In other words, the sum  $\sum_{\substack{(\beta, \gamma) \in \text{Comp} \times \text{Comp}; \\ \beta\gamma = \alpha; \\ \mu \in C(\beta); \\ v \in C(\gamma)}} u_{\mu, v}$  has exactly one addend. Hence, this

sum equals  $u_{\mu, v}$ . This proves Claim 1.]

*Claim 2:* Let  $(\mu, v) \in \text{Comp} \times \text{Comp}$  be such that  $\mu v \notin C(\alpha)$ . Then,

$$\sum_{\substack{(\beta, \gamma) \in \text{Comp} \times \text{Comp}; \\ \beta\gamma = \alpha; \\ \mu \in C(\beta); \\ v \in C(\gamma)}} u_{\mu, v} = 0.$$

[Proof of Claim 2: If  $(\beta, \gamma) \in \text{Comp} \times \text{Comp}$  is a pair of compositions satisfying  $\beta\gamma = \alpha$  and  $\mu \in C(\beta)$  and  $\nu \in C(\gamma)$ , then Proposition 5.15 shows that  $\mu\nu \in C\left(\underbrace{\beta\gamma}_{=\alpha}\right) = C(\alpha)$ , which contradicts  $\mu\nu \notin C(\alpha)$ . Hence, there exists no pair  $(\beta, \gamma) \in \text{Comp} \times \text{Comp}$  of compositions satisfying  $\beta\gamma = \alpha$  and  $\mu \in C(\beta)$  and  $\nu \in C(\gamma)$ . In other words, the sum  $\sum_{\substack{(\beta, \gamma) \in \text{Comp} \times \text{Comp}; \\ \beta\gamma = \alpha; \\ \mu \in C(\beta); \\ \nu \in C(\gamma)}} u_{\mu, \nu}$  is empty. Therefore, this

sum equals 0. This proves Claim 2.]

Now, each pair  $(\mu, \nu) \in \text{Comp} \times \text{Comp}$  satisfies either  $\mu\nu \in C(\alpha)$  or  $\mu\nu \notin C(\alpha)$  (but not both). Hence, we can split the outer sum on the right hand side of (35) as follows:

$$\begin{aligned}
& \sum_{(\mu, \nu) \in \text{Comp} \times \text{Comp}} \sum_{\substack{(\beta, \gamma) \in \text{Comp} \times \text{Comp}; \\ \beta\gamma = \alpha; \\ \mu \in C(\beta); \\ \nu \in C(\gamma)}} u_{\mu, \nu} \\
&= \sum_{\substack{(\mu, \nu) \in \text{Comp} \times \text{Comp}; \\ \mu\nu \in C(\alpha)}} \sum_{\substack{(\beta, \gamma) \in \text{Comp} \times \text{Comp}; \\ \beta\gamma = \alpha; \\ \mu \in C(\beta); \\ \nu \in C(\gamma)}} u_{\mu, \nu} + \sum_{\substack{(\mu, \nu) \in \text{Comp} \times \text{Comp}; \\ \mu\nu \notin C(\alpha)}} \sum_{\substack{(\beta, \gamma) \in \text{Comp} \times \text{Comp}; \\ \beta\gamma = \alpha; \\ \mu \in C(\beta); \\ \nu \in C(\gamma)}} u_{\mu, \nu} \\
&= \sum_{\substack{(\mu, \nu) \in \text{Comp} \times \text{Comp}; \\ \mu\nu \in C(\alpha)}} u_{\mu, \nu} + \underbrace{\sum_{\substack{(\mu, \nu) \in \text{Comp} \times \text{Comp}; \\ \mu\nu \notin C(\alpha)}} 0}_{\substack{= u_{\mu, \nu} \\ \text{(by Claim 1)}}} = \sum_{\substack{(\mu, \nu) \in \text{Comp} \times \text{Comp}; \\ \mu\nu \in C(\alpha)}} u_{\mu, \nu}.
\end{aligned}$$

Hence, we can rewrite (35) as

$$\sum_{\substack{(\beta, \gamma) \in \text{Comp} \times \text{Comp}; \\ \beta\gamma = \alpha}} \sum_{\mu \in C(\beta)} \sum_{\nu \in C(\gamma)} u_{\mu, \nu} = \sum_{\substack{(\mu, \nu) \in \text{Comp} \times \text{Comp}; \\ \mu\nu \in C(\alpha)}} u_{\mu, \nu}.$$

This proves Proposition 5.17. □

## References

- [Grinbe15] Darij Grinberg, *Double posets and the antipode of QSym*, arXiv:1509.08355v3.
- [GriVas22] Darij Grinberg, Ekaterina A. Vassilieva, *The enriched  $q$ -monomial basis of the quasisymmetric functions*, arXiv:?????.
